# Supplementary material for: Quantifying dynamics of failure across science, startups, and security
Source: arXiv:1903.07562 source file (2019-03-18)
Supplement: Supplementary file 1 [file Supp_N.pdf]

# Supplementary Information for Quantifying dynamics of failure across science, startups, and security

Yian Yin,[1,2] Yang Wang,[1,3] James A. Evans,[4,5] Dashun Wang[1,2,3]

[1] *Northwestern Institute on Complex Systems, Northwestern University, Evanston, IL 60208, USA*

[2] *McCormick School of Engineering, Northwestern University, Evanston, IL 60208, USA*

[3] *Kellogg School of Management, Northwestern University, Evanston, IL 60208, USA*

[4] *Department of Sociology, University of Chicago, Chicago, IL 60637, USA*

[5] *Santa Fe Institute, Santa Fe, NM 87501, USA*

# Contents

**S1 Data description** **3**

S1.1 NIH grant application dataset . . . 3
S1.2 VentureXpert investment dataset . . . 4
S1.3 GTD terrorism attack dataset . . . 6
S1.4 Data limitations . . . 7

**S2 Related work and models** **8**

S2.1 Learning literature . . . 8
S2.2 Stochastic models with memory . . . 8
S2.3 Adaptation models . . . 9
S2.4 Search models . . . 12
S2.5 Individual learning models . . . 14
S2.6 Urn models . . . 16
S2.7 Other models . . . 18

**S3 Modeling failure dynamics** **21**

S3.1 The $k$ model . . . . . . . . . . . . . . . . . . . . . . . . . . . . . . . . . . . 21
S3.2 Independent model ($k = 0$) . . . . . . . . . . . . . . . . . . . . . . . . . . . . 23
S3.3 Learning from all failures ($k \to \infty$) . . . . . . . . . . . . . . . . . . . . . . . . 23
S3.4 Solving the general model . . . . . . . . . . . . . . . . . . . . . . . . . . . . . 25
S3.5 Connections with canonical ensembles . . . . . . . . . . . . . . . . . . . . . . . 31
S3.6 Functional forms of $\rho(x)$ and $p(x)$ . . . . . . . . . . . . . . . . . . . . . . . . . 34
S3.7 Null models . . . . . . . . . . . . . . . . . . . . . . . . . . . . . . . . . . . . 36
S3.8 Failure streak length . . . . . . . . . . . . . . . . . . . . . . . . . . . . . . . . 38

**S4 Empirical measurements** **42**

S4.1 Quantifying performance dynamics . . . . . . . . . . . . . . . . . . . . . . . . 42
S4.2 Length distribution of failure streaks . . . . . . . . . . . . . . . . . . . . . . . 44
S4.3 Measuring failure dynamics . . . . . . . . . . . . . . . . . . . . . . . . . . . . 44

**S5 Prediction task** **46**

S5.1 Predicting ultimate success . . . . . . . . . . . . . . . . . . . . . . . . . . . . 46
S5.2 Testing power law model . . . . . . . . . . . . . . . . . . . . . . . . . . . . . 48

**S6 Robustness checks** **49**

S6.1 Definition of successes and failures . . . . . . . . . . . . . . . . . . . . . . . . 49
S6.2 Threshold for being inactive in the system . . . . . . . . . . . . . . . . . . . . . 49
S6.3 Comparing first failures versus halfway/penultimate failures . . . . . . . . . . . . 50
S6.4 Other checks . . . . . . . . . . . . . . . . . . . . . . . . . . . . . . . . . . . . 50

## S1 Data description

In this project, we compiled a comprehensive database consisting of three large-scale datasets across three different domains: Dataset $D_1$ contains submission histories of individual scientists in the US National Institutes of Health (NIH) grant system. $D_2$ contains profiles of innovators together with their startup ventures recorded in the VentureXpert investment database. $D_3$ records terrorist organizations and attacks retrieved from the Global Terrorism Database.

### S1.1 NIH grant application dataset

Our first dataset contains all R01 grant applications (776,721 in total) that have been ever submitted by 139,091 scientists to NIH from 1985 to 2015. For each grant application, we obtained its evaluation score (if reviewed on a panel), a unique identifier for the PI, the PI's name, and the application outcome (funded/not funded).

The NIH grant application dataset represents an excellent setting to study dynamics of failure for several reasons. First, it contains ground-truth information for both successes and failures. Second, as the world's largest public funder for biomedical research, NIH is the dominant funding source for biomedical scientists in the US[28,50]. Indeed we tracked funding acknowledgment information cited within biomedical research papers, finding among all PubMed papers published in the US (2008 to 2015), NIH indeed represents the majority of funding sources (81% out of top 10 agencies) (Fig. S1a).

R01 is the most common research funding mechanism within the NIH[26–28], accounting for the majority of the total funding. To compare the dynamical pattern between R01 and other granting mechanisms, we downloaded successful NIH grants from other mechanisms from NIH Research Portfolio Online Reporting Tools (RePORT), finding R01 grants are uniformly distributed within all NIH grants one obtains throughout a career (Fig. S1b).

Here we extract all new grant applications (excluding renewals, revisions and resubmissions) to reconstruct sequences of attempts (Fig. S2a). We truncate each sequence if (i) the individual gets one grant (success group, Fig. S2b); or (ii) the individual has been inactive for a long period (non-success group). Here we show results using all failure samples in main text. We also repeated our results using just the first sequence of failures—failure streak without prior success, finding our conclusions remain the same (Fig. S21,S22). We also find that the observed patterns are not affected by any potential periodicity of grant applications, and the results are robust against such variants. Indeed, we find the results remain the same if we add to timestamp of each attempt an artificial random noise at the scale of review cycles ($\sim$ 120 days).

### S1.2 VentureXpert investment dataset

Our second dataset traces start-up investment records from the VentureXpert (SDC Platinum) database, including 58,111 startup companies and 163,106 investment rounds from 1970 to 2016. For each investment we obtained information on investment amount, funding date, company name and a full list of innovators involved. We then link these records with company information on

Initial Public Offering and Merge & Acquisitions as outcome variables. Following definitions in entrepreneurship literature[30,31,51], we match individual entrepreneurs and startup ventures by linking each company with people listed as executives or board members at the first funding round. One advantage of this dataset is that 98.7% records have complete information of first and last names rather than initials, allowing us to construct career trajectories of 253,579 innovators.

Among the existing datasets capturing startups, the VentureXpert database, the official database of the National Venture Capital Association is among the most comprehensive and authoritative databases[29]. To further explore the coverage of the database, we compare the number of IPOs within our data versus US total counts, finding our dataset captures a significant fractions of IPOs, with the ratio between the two statistics remaining stable across time (Fig. S3), documenting the reliability of this dataset. We also cross-validated individual entrepreneurs coverage with Crunchbase, an online platform of business information. We select top 1000 serial executives and board members ranked by the number of different jobs in Crunchbase, finding more than 70% of the profiles are included in VentureXpert as well. Overall, these statistics document that our dataset has excellent coverage through various validation efforts.

Another challenge in modeling dynamics of failure in startup datasets is the ambiguity of 'failures'[52], which could include bankruptcy, termination to prevent future losses, and deviation from desired results. Recognizing the complexity of this issue, here we closely follow existing literature on venture capital and serial entrepreneurship[30,31]. We focus on all portfolio companies that have received at least one round of funding, and define those who went public or get acquired

or merged at high values (percentile as compared with all M&As in the same year) as successes. We performed different variants of measurements by changing the percentile threshold (1% and 5%) and also by only including IPO (Figs. S24,S25). We find our results remain the same. If a company obtained its first investment but did not succeed within a certain period, this venture is marked as a failure. In this dataset we treat each new venture as an attempt, starting at the date of first round investment. Similar to $D_1$, sequences of attempts by each individual are collected into a sequence, where the stopping criterion is defined by (i) the individual has one company that eventually achieved IPO or high-value M&As (success-group); (ii) the individual has been inactive for a long period without success (non-success group).

### S1.3 GTD terrorism attack dataset

Our third dataset contains 170,350 terrorist attacks by 3,178 organizations from 1970 to 2017, collected by the Global Terrorism Database, one of the most systematic databases on domestic and transnational terrorist events[32]. For each attack we obtain information on its date, type, location, and consequences in terms of the number of people killed and wounded. Some records in this corpus are based on speculation or dubious claims of responsibility, which are discarded in our analysis to ensure the data quality.

There lacks a clear definition of 'success' for terrorist attacks, partly due to their diverse intents and consequences. To be consistent with our empirical steps in $D_1$ and $D_2$, here we treat an attack as successful if it killed at least one victim. One potential concern of this definition

is that goals of terrorism attacks differ, and not all attacks are aimed at killing victims. This concern is somewhat alleviated, however, as 84.7% the attacks are indeed targeted at human beings (i.e. assassination, bombing/explosion and assault). We further performed robustness checks by focusing on these types of attacks (Fig. S26), finding our results remain the same. Therefore we collected sequences of attacks of each terrorist organization. We classify the samples if (i) the organization killed at least one people (success group); (ii) the organization has been inactive for a long period without success (non-success group).

### S1.4 Data limitations

Our data are not without limitations. For example, as agents who failed may change their goals and subsequently transfer to other systems, it is difficult to obtain the full coverage of all attempts. For example, one might apply for grants from other funding agencies, found startup ventures without VC investments, or stop launching terrorist attacks for other activities. While our systematic validation efforts in S1.1-S1.3 have not uncovered any potential biases, readers should keep in mind of the existence of such factors. Nevertheless, despite these potential limitations, it is important to note that the three data sources are among the largest in their respective domains, hence representing the state-of-art empirical corpora to understand failures.

## S2 Related work and models

### S2.1 Learning literature

This paper is closely related to the rich literature on learning and failures. Canonical frameworks in understanding how people react to failures[19,38,52–56] have identified several key factors that could impact learning, including individual characteristics and organizational structures and strategies. These findings have also prompted quantitative studies using failure records across different industries, ranging from entrepreneurship[30,31] to commercial banking[57], from healthcare[58] to coal mining[59] to trains[60], and airlines[61] to orbital launch vehicles[62].

Another relevant line of inquiry is in psychology and organization behavior, which concerns learning curves from both theoretical[18–23,33,34,37–39,42,43,63–65] and empirical[21,37–40,44,66] perspectives, quantifying how performance and efficiency improve with experience. One key result is the famous Wright's law[44], i.e. the power law form of cost reduction.

Next we review a series of major models and compare key predictions with our empirical results. We summarize all these models in Table S1.

### S2.2 Stochastic models with memory

One school of thought can be viewed as modeling the dependence structure among failures. Indeed, the failure of the chance model suggests that non-trivial dependence may be essential for modeling

the fat-tailed length distribution of failure streaks, which raises an important question: Could other stochastic processes (Markov process, random walk, autoregressive model, etc.) account for our observations? Indeed, if we consider a general framework of fixed dependence as follows

$$S_n = f_n(S_1, S_2, \cdots, S_{n-1}), \tag{S1}$$

where $S_n$ denotes the performance at the $n$-th attempt and $f_n$ can be a deterministic or stochastic non-decreasing mapping. This framework covers a wide range of stochastic processes, e.g. $f_n(S_1, \cdots, S_{n-1}) = f_n(S_{n-1})$ for a discrete space of $S_n$ leads to Markov process, $f_n(S_1, \cdots, S_{n-1}) = S_{n-1} + \epsilon_n$ leads to random walk, $f_n(S_1, \cdots, S_{n-1}) = \sum_{i=1}^{p} \phi_i S_{n-i} + \epsilon_n$ leads to autoregressive model. We note that if this is true, we can obtain

$$S_n = f_n(S_1, f_1(S_1), \cdots, f_{n-1}(S_1, f_1(S_1), \cdots)) \equiv g_n(f_1, \cdots, f_n)(S_1) \tag{S2}$$

Hence, $S_n$ can be formulated as a non-decreasing function of $S_1$, indicating that there should be detectable 'fitness' differences in the first attempt. Indeed, these results indicate that if there exists no difference in the dependency structure $f_n$, the differences in outcomes should be at least partly contributed by performance at the first attempt, which contradicts with our data. This hypothesis also cannot explain the fat-tail length distribution of failure streaks (S3.8).

### S2.3 Adaptation models

The evolutionary perspective for individual and organizational learning assumes that the agent improves through updating information and belief on different alternatives. Here we discuss three representative models, each assuming a finite pool of available options.

#### S2.3.1 Crossman's model

Crossman's model, first proposed in[67], aims to explain the temporal scaling observed in individual tasks. The model suggests a process from $r$ methods $M_i$ ($1 \leq i \leq r$), each with a time cost $t_i$. The individual improves operation strategy through changing probabilities for using different methods, i.e. $p_i$ where $\sum_{i=1}^{r} p_i = 1$. At the $n$-th trial, the expected time cost can be formulated as

$$T(n) = \sum_{i=1}^{r} t_i p_i(n) \tag{S3}$$

The change of probability for choosing method $M_i$ is proportional to the difference between its time cost and current average time cost, i.e.

$$p_i(n+1) - p_i(n) = -k(t_i - T(n)) \tag{S4}$$

Therefore, the time cost decays as

$$T(n+1) = T(n) - k \sum_{i=1}^{r} p_i (t_i - T(n))^2 \tag{S5}$$

#### S2.3.2 NK model

NK model, initially proposed by Kauffman[68] is a canonical model in organizational learning[69]. Consider a rugged fitness space of $N$ dimensions $X = (x_1, \cdots, x_N)$, where $x_i \in \{0, 1\}$. The fitness score of each possibility is the summation of interaction among $K$ adjacent dimensions, that writes

$$\phi(x) = \sum_{i=1}^{N} \phi_i(x_i, \cdots, x_{i+K}) \tag{S6}$$

One heuristic searching strategy in this rugged landscape concerns two options:

(1) Local search, i.e., walk to a neighbor, $y$, which satisfies $|y - x| = 1$.

(2) Global search, i.e., jump to a new node randomly.

#### S2.3.3 Denrell and March's model

Denrell and March proposed a simple adaptation model to understand the interplay between information and adaptation, explaining why people have bias against novel and risky choices[70]. In this model, $P_t$, defined as the probability for the first option to be chosen at time $t$, depends on its past probability $P_{t-1}$ and current performance. If the option leads to better outcome compared with the other, one updates

$$P_{t+1} = P_t + a(1 - P_t) \tag{S7}$$

otherwise,

$$P_{t+1} = (1 - a)P_t \tag{S8}$$

All three models presented here can mimic specific performance or efficiency trajectory as one tries repeatedly. The main issue with these models is that they all base on a finite space of possible options, which leads to a limit in performance and efficiency improvement that one cannot overcome, which contradicts with our data.

### S2.4 Search models

Search models assume an iterative process, where one decides whether to use existing components or try new ones based on component quality. Such models are often characterized by an improvement in the objective performance function because of the extreme values theory, i.e. as one always selects the best version from experimentation, she will eventually arrive at the version that is reasonably good.

#### S2.4.1 Roberts' model

Robert proposed a model based on greedy algorithms[64]. To understand the universal learning process, the model assumes production efficiency $p$ as lognormal, following

$$x = b \ln p \tag{S9}$$

where $x$ follows the standard normal distribution $N(0, 1)$. Each time the agent randomly selects a sample $x'$ and compares it with current efficiency $x$, adopting the new method when $x' < x - a$. The model predicts

$$\ln p \sim \ln N/ab \tag{S10}$$

#### S2.4.2 Muth's model

Muth's model[42] builds on a simple assumption: the individual tries a new method at each trial and uses the new method if it costs less. The model further assumes appropriate regularity conditions

for the cdf of cost $F$, e.g.

$$\lim_{x \to x_0} \frac{F(x)}{(x - x_0)^k} = c \tag{S11}$$

where $x_0$ is the limiting cost of production. The model predicts the expected cost $E[X_n]$ of the $n$-th production as

$$E[X_n] = x_0 + \Gamma(1 + 1/k)(cn)^{-1/k} \tag{S12}$$

Muth's model is an elegant model explaining the emergence of power law scaling and can be extended to dependent component cases.

### S2.4.3 McNerney's model

McNerney et al further extended Muth's model by assuming a power law distribution of costs of each component ($f(c_i) \sim x_i^{\gamma-1}$) and using design structure matrix to characterize the dependency among different components[43]. The model predicts the cost $y$ decreases as a function of productions $n$ following

$$y(n) \sim n^{-1/\gamma d^*} \tag{S13}$$

where $d^*$ is the design complexity and equals to 1 when all components are independent.

Search models successfully explain the emergence of power-law scaling in repeated attempts and serve as the basis of our frameworks (e.g. $k \to \infty$ limit). Yet they cannot account for the co-existence of two groups and their diverging patterns.

### S2.5 Individual learning models

There has also been an active line of inquiry in explaining practice curves in individual tasks[40,41,45,71]. These models use psychology models as well as cognitive theories to explain 'practice makes perfect'.

#### S2.5.1 Newell and Rosenbloom's chunking model

To explain the power-law scaling observed in human task performance, e.g. inverted text reading and ten-finger game, Newell and Rosenbloom modeled the learning process using chunking theory[40]. In this model, there is a tree structure for goal hierarchies of height $H$ and the speed-up of task completing is due to the emergence of higher-order chunks. The current highest order of chunk is denoted as $\eta$, leading to

$$\frac{dT}{dN} = \frac{dT}{d\eta}\frac{d\eta}{dN} \tag{S14}$$

The model further assumes each non-terminal goal has $\beta$ non-terminal subgoals and $\omega$ terminal subgoals. As one constructs chunks of higher levels, the corresponding time to perform a new attempt decreases exponentially following

$$\frac{dT}{d\eta} \sim \beta^{H-\eta} \tag{S15}$$

If we also assume the chunking rate is linear with respect to time and the birth of a single level-$h$ chunk requires time $s(h)$, we have

$$\frac{d\eta}{dN} \sim \frac{\beta^{\eta-H}}{s(\eta)}T \tag{S16}$$

Therefore, if $s(\eta)$, the number of possible states for goals at level $\eta$ (complexity at this level), takes an exponential form as $s(\eta) \sim e^{\alpha\eta}$, which is consistent with the tree structure, we have

$$\frac{dT}{dN} \sim \frac{(T+E)^{-x}}{T} \tag{S17}$$

which follows a power law scaling. Hence, by combining two exponential forms in a tree structure, the authors successfully derive the power law scaling.

#### S2.5.2 Anderson's model

Based on ACT's strengthening process, Anderson developed a model explaining cost decay[41]. The model assumes the amount of practice as $S$ and the production execution in ACT takes the form

$$T = c + aS^{-1} \tag{S18}$$

The amount of past practice also decays as a power law of practice time:

$$S = \sum_{i=0}^{P-1} s(i,P) \sim \sum_{i=1}^{P} i^{-d} \sim P^{1-d} \tag{S19}$$

Therefore, we have

$$T = C' + A'P^{d-1} \tag{S20}$$

The two models are very relevant to our settings and can predict power law temporal scaling in the success group. They represent two fundamental classes of cognitive architectures in related studies: ACT and Soar (and their variants)[49], highlighting the role of memory and chunks in learning process. Yet such mechanisms are more appropriate for modeling simple tasks rather than complex innovative ones and cannot account for the co-emergence of success and non-success groups.

### S2.6 Urn models

Urn model and its variants are among the canonical models in social physics as well as innovation process[72]. This model family is closely related to the famous Heaps' law[73], originally predicting that the number of distinct words $S$ in a paragraph of length $n$ scales as

$$S(n) \sim n^{\beta}, \;\; 0 < \beta \leq 1 \tag{S21}$$

Note that if we assume generating a new word costs unit time, we know the expected time spent on the $n$-th 'word' follows

$$t_n \sim n^{\beta-1} \equiv n^{-\gamma}, \;\; 0 < \gamma \leq 1 \tag{S22}$$

which recovers our empirical findings. Here we review several generative models explaining this scaling.

#### S2.6.1 Simon's model

Simon's model is among the earliest frameworks modeling 'cumulative advantages'[74]. It assumes that (1) There is always constant probability $p$ for an agent to take a new word for the next element; (2) Otherwise (with probability $1-p$) the agent reuses past words based on frequency, i.e. randomly select a word from the past sequence. This model predicts a linear scaling between $S$ and $n$ i.e. $\beta = 1$, which can only explain the emergence of the non-success group.

#### S2.6.2 Tria's model

By extending studies on urn model, Tria et al[75] assume an urn $U$ of ideas and a sequence of $S$ to generate. Every time an element is sampled from $U$ to $S$, $\rho$ copies are put back to $U$. Further, if this sampled idea is new in $S$, it triggers $\nu$ adjacent new ideas, hence the number of different ideas in a sequence follows the master equation

$$\frac{dD}{dt} \approx \frac{\nu D}{\rho t + (\nu + 1)D} \tag{S23}$$

The solution reveals that $D$ grows linearly with $t$ for $\nu > \rho$, but follows Heaps' law $D \sim t^{\nu/\rho}$ for $\nu < \rho$. These predictions are similar to the first phase transition point $k^*$ in our model.

#### S2.6.3 Iacopini's model

To further document the impact of past transition sequence in innovative attempts, a recent paper[76] proposed a network-based model, where ideas are represented as nodes, and one can travel from one idea to another when they are linked by a weight. The process is set to be a weighted random walk on networks, following

$$P^t(i \to j) = \frac{w_{ij}^t}{\sum_k w_{ik}^t} \tag{S24}$$

When a specific path $i \to j$ is traveled, the weight of this edge is updated

$$w_{ij}^{t+1} = w_{ij}^t + \delta w \tag{S25}$$

Depending on different network structures, the model can lead to scaling $S \sim n^\beta$ with varying $\beta$.

While this class of models does not capture the performance dynamics underlying failures,

they are highly relevant to our study in that their predictions are consistent with the temporal patterns observed in our data.

### S2.7 Other models

#### S2.7.1 Levy's model

Levy modeled the improvement of productivity based on the limited range of output denoted as $P$[39]. Given the current rate of production after producing $q$ items, $Q(q)$, the improvement of production rate is proportional to the amount that the process can improve, i.e.

$$\frac{dQ(q)}{dq} = \mu[P - Q(q)] \tag{S26}$$

leading to

$$Q(q) = P[1 - e^{a+\mu q}] \tag{S27}$$

Levy's model captures a kind of production process where the final plateau part is significant, but it fails to predict the power-law form of productivity improvement.

#### S2.7.2 Shrager's model

By collecting and analyzing data of path length in the bit game, Shrager et al developed a graph-dynamic model for route-finding in ER networks $G(n, p)$[22]. The authors proposed a strategy where the individual randomly selects an edge after deleting the ones moving away from the destination with probability $r$. The number of trials increases the network density $p$ linearly and the cost is the

path length of the whole process $s$. For $r$ near 0, the model predicts

$$s \sim \frac{2}{p}(1-r)^{\ln n/\ln(np)} \tag{S28}$$

while for $r$ near 1, the model predicts

$$s \sim \ln n/\ln(np) \tag{S29}$$

### S2.7.3 Sahal's model

Sahal explains the progress function in industry productions through probabilistic and deterministic models[63]. The model assumes different manpower levels and $X(s,t)$ to be the number of product quantities requiring $s$ amount of manpower at time $t$. If we assume the improvement across $u$ manpower levels does not depend on the current level and can be formulated as $p(u)$, yielding

$$X(s,t+1) = \sum_{u=-n}^{1} X(s-u,t)p(u) \tag{S30}$$

If we define $X(s) = \lim_{t\to\infty} X(s,t)$, the solution of this equation can be formulated as

$$X(s) = b^s,\ 0 < b < 1 \tag{S31}$$

The model further assumes levels manpower are distributed on a logarithmic scale with width $h$, obtaining

$$F(Y) \sim Y^{-\log b/h} \tag{S32}$$

where $F(Y)$ is the number of product quantities requiring manpower greater than $Y$.

### S2.7.4 Johnson's model

Johnson et al reported a similar scaling from the time interval of terrorist attacks and other human confrontations[34]. An illustrative model for this scenario considers confrontation between 'Red Queen' and 'Blue King', and the advantage of Red Queen after $n$ events, $R(n)$, can be formulated as

$$R(n) = \sum_{i=1}^{n} x_i \tag{S33}$$

where $x_i$ takes value $+d$ or $-d$ with probability 1/2. Depending on the auto-correlation of $x_i$, one can get

$$R(n) \sim n^b d, 0 \leq b \leq 1 \tag{S34}$$

Taking the inverse of the advantage, we get the attack rate scales as a negative power law of $n$, i.e.

$$\tau_n \sim n^{-b}, 0 \leq b \leq 1 \tag{S35}$$

### S2.7.5 Clauset's model

Clauset's model[33] also aims at understanding the temporal pattern of terrorist attacks, but in a very different way from Johnson's model[34]. Indeed, it is found that the size of terrorism organizations scales linearly with its past attacks, i.e.

$$s(n+1) = s(n) + \eta \tag{S36}$$

The model further assumes a new takes time as the inverse of organization size, i.e.

$$\Delta t \sim 1/s \tag{S37}$$

Taken together, we have

$$\Delta t \sim 1/n \tag{S38}$$

Therefore, this model only applied to group dynamics and the exponent of power law is restricted to be -1.

One commonality among these models is that they lack predictions of the interplay between performance and time. By contrast, our data show that the temporal scaling cannot be simply explained by agents optimizing time cost $t_n$ since the performance also improves for the success group. These models also cannot explain the co-existence of success and non-success groups observed in our data.

## S3 Modeling failure dynamics

### S3.1 The $k$ model

In order to formulate a new attempt, the individual needs to go through every component, and decide what to do next. For a past attempt $j$, each component $i$ is characterized by an evaluation score $x_j^{(i)}$, which falls between 0 and 1. The agent can either create a new version (with probability $p$), or with probability $1-p$ reuse an old one by choosing among past versions. The main cost of creating a new version is time. Here we assume each new version takes one unit of time, and upon creation takes up an evaluation score, drawn randomly from a fixed distribution $\rho(x)$. Real systems are likely to differ in their specific score distributions. Here for simplicity, we assume $\rho(x)$ follows a uniform distribution on $[0, 1]$, approximating the percentile of any underlying score

distributions real systems may follow. One difference between our model and canonical learning curve models[43] is that one has little information on the new versions until it gets implemented and evaluated, hence new versions are not guaranteed to increase or decrease their score.

Of the many factors that may influence $p$, one key factor is the quality of existing versions. Denoting with $x^*$ the best score among past versions, we expect $p$ to be a function of $x^*$. Indeed, consider the two extreme cases. If $x^* \to 0$, existing versions of this component have among the worst scores hence a high potential to be improved upon with a new version. Therefore the likelihood of creating a new version is high, i.e., $p \to 1$. On the other hand, $x^* \to 1$ indicates an already excellent version, corresponding to a decreased incentive to create a new one ($p \to 0$). Reusing the existing best version allows the particular component to retain its score $x^*$ and also avoids incurring additional time cost the individual can avoid spending time working on. To this end, considering $P(x \geq x^*) = 1 - x^*$ as the potential to improve on existing versions, we assume $p = (1 - x^*)^\alpha$, where $\alpha > 0$ characterizes an individual's propensity to create new versions given the quality of existing versions. The higher this potential, the more likely one may create a new version[70].

The dynamics of quality score, $x_n$, can be captured by a higher-order Markov process of memory length $k$, following

$$x_n^* = \max\{x_{n-k}, \cdots, x_{n-1}\} \tag{S39}$$

$$x_n \sim \begin{cases} U[0,1], & w.p.\ (1 - x_n^*)^\alpha \\ \delta(x_n^*), & w.p.\ 1 - (1 - x_n^*)^\alpha \end{cases} \tag{S40}$$

where we assume $x_n = 0$ for all $n < 0$. Directly solving the model is extremely difficult, given the increasing complexity brought by the higher-order dependencies as well as the continuous state space, which eventually lead to the rich mathematical phenomenon documented in Fig. 3. We can, however, first look at two extreme cases that are more tractable.

### S3.2 Independent model ($k = 0$)

Here we first consider a simple case when $k = 0$, i.e. there lacks any reusable materials in memory as one tries again. In this case, one creates a new version every time, hence for all $n$ we have

$$x_n \sim U[0, 1] \tag{S41}$$

and

$$t_n \equiv 1 \tag{S42}$$

### S3.3 Learning from all failures ($k \to \infty$)

We now turn to another extreme: learn from all past failures. We can rewrite the process as

$$x_n^* = \max\{x_0, \cdots, x_{n-1}\} \tag{S43}$$

$$x_n \sim \begin{cases} U[0,1], & w.p.\ (1 - x_n^*)^\alpha \\ \delta(x_n^*), & w.p.\ 1 - (1 - x_n^*)^\alpha \end{cases} \tag{S44}$$

Here we focus on the dynamics of $x^*$, obtaining

$$x^*_{n+1} \sim \begin{cases} U[0, x^*_n], & w.p.\ (1-x^*_n)^{\alpha+1} \\ \\ \delta(x^*_n), & w.p.\ 1-(1-x^*_n)^{\alpha+1} \end{cases} \tag{S45}$$

where $x^*_1 \sim U[0,1]$. To this end, let us denote $f_n$ as the probability density function of $x^*_n$, we obtain

$$f_{n+1}(x) = f_n(x)(1-(1-x)^{\alpha+1}) + \int_0^x f_n(y)(1-y)^\alpha dy \tag{S46}$$

with $f_1(x) \equiv 1$ for $x \in [0,1]$. By induction we obtain

$$f_n(x) \sim [1-(1-x^{\alpha+1})]^{n-1} \tag{S47}$$

The normalization constant equals to

$$\int_0^1 [1-(1-x)^{\alpha+1}]^{n-1}dx = \int_0^1 (1-x^{\alpha+1})^{n-1}dx = \int_0^1 x^{-\alpha}(1-x^{\alpha+1})^{n-1}dx^{\alpha+1}/(\alpha+1) = B(n,1/(\alpha+1))/(\alpha+1)$$

Therefore we have

$$\begin{aligned} t_n &= \frac{\int_0^1 (1-x)^\alpha f_n(x)dx}{\int_0^1 f_n(x)dx} \\ &= \frac{B(n,1)}{B(n,1/(\alpha+1))} \\ &\sim \frac{\Gamma(1)n^{-1}}{\Gamma(1/(\alpha+1))n^{-1/(\alpha+1)}} \\ &\sim \Gamma\left(\frac{1}{\alpha+1}\right)^{-1} n^{-\frac{\alpha}{\alpha+1}} \end{aligned} \tag{S48}$$

and

$$
\begin{aligned}
1-x_n &= \frac{\int_0^1\{(1-x)[1-(1-x)^\alpha)]+(1-x)^\alpha/2\}f_n(x)dx}{\int_0^1 f_n(x)dx} \\
&= \frac{B(n,2/(\alpha+1))-B(n,1+1/(\alpha+1))+B(n,1)/2}{B(n,1/(\alpha+1))} \\
&\sim \frac{\Gamma(2/(\alpha+1))n^{-2/(\alpha+1)}-\Gamma(1+1/(\alpha+1))n^{-1-1/(\alpha+1)}+\Gamma(1)n^{-1}/2}{\Gamma(1/(\alpha+1))n^{-1/(\alpha+1)}} \\
&\sim \Gamma\left(\frac{1+\min\{\alpha,1\}}{\alpha+1}\right)\Gamma\left(\frac{1}{\alpha+1}\right)^{-1} n^{-\frac{\min\{\alpha,1\}}{\alpha+1}}
\end{aligned}
\tag{S49}
$$

Hence, both efficiency and quality scales with $n$, following $\gamma = 1-1/(\alpha+1)$ and $\eta = \min\{\gamma, 1-\gamma\}$.

### S3.4 Solving the general model

We note that the previous two cases are tractable because either $x_n$ or $x_n^*$ can be formulated into a simple Markov process without higher-order dependencies. However, such techniques cannot be directly applied to general cases. As will be shown below, by using renewal process theories[36], we can successfully obtain accurate values of scaling exponents (Fig. S7). We first note that

$$|\{n_1 \le n \le n_2 : x_n = x_m^*\}| \le n_2 - n_1 + 1 \tag{S50}$$

$$|\{n_1 \le n \le n_2 : x_n = x_m^*\}| \ge \sum_{i=0}^{[(n_2-n_1)/k]-1} \sum_{j=0}^{k-1} I(x_{n_1+ki+j} = x_{n_1+ki+i}^*) \ge [(n_2-n_1)/k] \tag{S51}$$

Hence to calculate the length of a sequence, we only need to estimate the number of versions that are once baseline versions (i.e. $n$ such that $x_n = x_m^*$ for some $n+1 \le m \le n+k$).

Denote $z_m = 1 - x_n^*$ as all such baseline scores. We now calculate for a specific $z_m$ to be taken by a new one, the number of attempts it takes. Indeed, given a score $z_m$ and assuming that it

has been reused as $z_m = z_{m-1}$, we have

$$z_{m+1} = \begin{cases} z_m & w.p.\ \frac{[1-z_m^{k\alpha}(1-z_m)^k](1-z_m^{\alpha})}{1-z_m^{\alpha}(1-z_m)} \sim O(1) \\ U[0, z_m] & w.p.\ \frac{[1-z_m^{k\alpha}(1-z_m)^k]z_m^{\alpha+1}}{1-z_m^{\alpha}(1-z_m)} \sim O(z_m^{\alpha+1}) \\ \min\{U_1[0,1], \cdots, U_k[0,1]\} & w.p.\ z_m^{k\alpha}(1-z_m)^k \sim O(z_m^{k\alpha}) \end{cases} \quad \text{(S52)}$$

Here we use the big-O notation to find the asymptotic case for $z_m \to 0$, the only limit that could possibly exist divergence leading to emergence of scaling and phase transitions. This equation shows two important insights:

(1) If we calculate the number of iterations that $z_m$ gets reused, it should be in the order of $O(z_m^{-\min\{k\alpha,\alpha+1\}})$, leading to two cases that will be discussed in detail.

(2) There exist two different mechanisms driving the substitution of baseline versions: *Quality* ($w.p.\ O(z^{k\alpha})$) and *Recency* ($w.p.\ O(z^{\alpha+1})$). For $k\alpha < \alpha + 1$, the recency mechanism takes the majority for small $z$, i.e. produces a worse succeeding score. Hence, it keeps an equilibrium of score as $n$ increases. However, once $k\alpha > \alpha + 1$, quality mechanism takes over for small $z$, characterizing a continuous path of getting better and better.

Here, we first derive our results for the regime $k\alpha < \alpha + 1$, and extend the obtained results to the other regime.

### S3.4.1 Case 1: $k\alpha < \alpha + 1$

When $z_{m+1} \neq z_m$, our previous results show that with high probability, $z_m$ is the extreme value among $k$ i.i.d. random variables on $U[0,1]$, hence the pdf of $z_m$, $f(z_m) \sim const$ as $z_m \to 0$. Below we offer a more rigorous proof: Here we take all the different $z_m$ as $\tilde{z}$ and consider a limiting distribution of $f(\tilde{z})$, we have

$$f(\tilde{z}) \sim \int_0^1 f(\tilde{z}')O(1)d\tilde{z}' + \int_{\tilde{z}}^1 f(\tilde{z}')O(\tilde{z}'^{\alpha+1-k\alpha})/\tilde{z}'d\tilde{z}' \tag{S53}$$

Assuming $f(\tilde{z}) \sim \tilde{z}^{\beta_1}$ and consider $\tilde{z} \to 0$ one gets

$$\beta_1 = \min\{0, 1, \beta_1 + \alpha + 1 - k\alpha\} = \min\{0, \beta_1 + \alpha + 1 - k\alpha\} \tag{S54}$$

Since $k\alpha < \alpha + 1$, we get $\beta_1 = 0$. Hence, as we generate a new baseline score satisfying $z_m \neq z_{m-1}$, we approximate the number of iterations it will be retained as $u \sim z^{-k\alpha}$. Let $z_m = z_{m+1} = \cdots = z_{m+u}$, while for $z_{m+u+1}$ we take a new random variable from a fixed distribution on $[0,1]$ whose probability density not diverge near 0. If we consider the change of baseline scores as a 'jump' and number of iterations of repeated reuse as the length of this jump ($u$), we eventually arrive at a Levy flight.

Define $u_i \equiv z_i^{-k\alpha}$, following asymptotically power law pdf $P(u) \sim u^{-1/k\alpha-1} \equiv u^{-\mu-1}$, define $m(N) = \min_m\{u_1 + \cdots u_m \geq N\}$. Next we solve $\langle u^\lambda_{m(N)} \rangle$ for some $\lambda$. We first calculate $P(u_{m(N)})$, which equals to

$$\begin{aligned} P(u_{m(N)} = u) &= P(u) \int_{\max\{N-u,0\}}^N \sum_{k=0}^{\infty} P_k(v)dv \\ &= P(u) \int_{\max\{N-u,0\}}^N G(v)dv \end{aligned} \tag{S55}$$

where $P_k(v) \equiv P(v_1 + \cdots + v_k = v)$ and $G(v) \equiv \sum_{k=0}^{\infty} P_k(v)$. $P_k$ can be analytically obtained by induction, following

$$P_k = \begin{cases} P_{k-1} \circ P, & k \leq 1 \\ \delta(0), & k = 0 \end{cases} \tag{S56}$$

Hence we have

$$G = \sum_{k=0}^{\infty} P_k = G \circ P + \delta(0) \tag{S57}$$

Taking the Laplace transformation we obtain

$$\tilde{G} = \tilde{G}\tilde{P} + 1 \tag{S58}$$

leading to

$$\tilde{G} = \frac{1}{1 - \tilde{P}} \tag{S59}$$

The quantity of interest, $M(N) \equiv \langle u^{\lambda}_{m(N)} \rangle$, can be formulated as

$$\begin{aligned} M(N) &= \int_0^{\infty} P(u_{m(N)} = u) u^{\lambda} \\ &= \int_0^N P(u) u^{\lambda} \int_{N-u}^N G(v) dv du + \int_N^{\infty} P(u) u^{\lambda} \int_0^N G(v) dv du \\ &= \int_0^N Q(u)[H(N) - H(N-u)] du + \int_N^{\infty} Q(u) H(N) du \\ &= H(N) \int_0^{\infty} Q(u) du - \int_0^N Q(u) H(N-u) du \\ &= H(N) \int_0^{\infty} Q(u) du - (Q \circ H)(N) \end{aligned} \tag{S60}$$

where $H(N) = \int_0^N G(v) dv$ and $Q(u) = u^{\lambda} P(u)$. Let us again perform the Laplace transforma-

tion, obtaining

$$
\begin{aligned}
\tilde{M} &= \tilde{H}(\int_0^\infty Q(u)du - \tilde{Q}) \\
&= \tilde{G}(\int_0^\infty Q(u)du - \tilde{Q})/s \\
&= \frac{\int_0^\infty Q(u)du - \tilde{Q}}{s(1-\tilde{P})}
\end{aligned}
\tag{S61}
$$

Assuming

$$
P(x) = \mu x^{-\mu-1} I(x \geq 1) \tag{S62}
$$

we obtain

$$
\tilde{P}(s) = \mu s^{\mu} \Gamma(-\mu, s) \tag{S63}
$$

$$
\tilde{Q}(s) = \mu s^{\mu-\lambda} \Gamma(\lambda - \mu, s) \tag{S64}
$$

$$
\int_0^\infty Q(u)du = \frac{\mu}{\mu - \lambda} \tag{S65}
$$

where $\Gamma(a, s) = \int_s^\infty t^{a-1} e^{-t} dt$ is the upper incomplete Gamma function. Inserting these results into the previous function we arrive at

$$
\tilde{M} = \frac{\mu/(\mu-\lambda) - \mu s^{\mu-\lambda} \Gamma(\lambda - \mu, s)}{s[1 - \mu s^{\mu} \Gamma(-\mu, s)]} \tag{S66}
$$

To obtain asymptotic results for $M(N)$ as $N \to \infty$, we approximate $\tilde{M}(s)$ as $s \to 0^+$. Here we use the following expansion

$$
\Gamma(a, s) = \Gamma(a) - \frac{s^a}{a} + \frac{s^{a+1}}{a+1} + O(s^{a+2}) \tag{S67}
$$

The previous equation hence writes

$$\begin{aligned}\tilde{M} &\approx \frac{\mu/(\mu-\lambda) - \mu s^{\mu-\lambda}\Gamma(\mu-\lambda) + \mu s^{\mu-\lambda}s^{\lambda-\mu}/(\lambda-\mu) - \mu s^{\mu-\lambda}s^{\lambda-\mu+1}/(\lambda-\mu+1)}{s[1-\mu s^{\mu}\Gamma(\mu) + \mu s^{\mu}s^{-\mu}/(-\mu) - \mu s^{\mu}s^{-\mu+1}/(1-\mu)]} \\ &= \frac{-\mu s^{\mu-\lambda}\Gamma(\mu-\lambda) - \mu s/(\lambda-\mu+1)}{s[-\mu s^{\mu}\Gamma(\mu) - \mu s^{\mu}s^{-\mu+1}/(1-\mu)]} \\ &= \frac{s^{\mu-\lambda}\Gamma(\mu-\lambda) + s/(\lambda-\mu+1)}{s[s^{\mu}\Gamma(\mu) + s/(1-\mu)]} \sim s^{\min\{\mu-\lambda,1\}-\min\{\mu,1\}-1}\end{aligned} \tag{S68}$$

Hence we obtain

$$M = L^{-1}(\tilde{M}) \sim n^{-\min\{\mu-\lambda,1\}+\min\{\mu,1\}} \tag{S69}$$

Let us consider the two specific cases:

Case 1: $\lambda = -1/k$, we have $M \sim n^{\min\{1/(k\alpha),1\}-1}$, hence

$$\langle (1-x^*)^{\alpha}\rangle \approx M = \begin{cases} \text{const.}, & k\alpha \le 1 \\ n^{-1+1/(k\alpha)}, & k\alpha > 1 \end{cases} \tag{S70}$$

Case 2: $\lambda = -1/(k\alpha)$, we have $M \sim n^{\min\{1/(k\alpha),1\}-\min\{2/(k\alpha),1\}}$, hence

$$\langle 1-x^*\rangle \approx M = \begin{cases} \text{const.}, & k\alpha \le 1 \\ n^{-1+1/(k\alpha)}, & 1 < k\alpha \le 2 \\ n^{-1/(k\alpha)}, & k\alpha > 2 \end{cases} \tag{S71}$$

This eventually leads to

$$\langle 1-x\rangle = \langle z\rangle = \langle z^* + z^{*\alpha}/2 - z^{*(\alpha+1)}\rangle \approx \langle z^* + z^{*\alpha}/2\rangle \sim n^{-\min\{1,k\alpha-1\}/k\alpha} \sim n^{-\min\{\gamma,1-\gamma\}} \tag{S72}$$

### S3.4.2 Case 2: $k\alpha > \alpha + 1$

As we solved previously, in this regime the quality dynamics is dominated by the second mechanism, which does not depend on $k$ any more, and should be asymptotically the same as learning

from all failures model ($k = \infty$). Indeed, if we expand our solution and take $k \to (1 + 1/\alpha)^-$, we obtain $\gamma = 1 - 1/(k\alpha) \to \alpha/(\alpha + 1)$ and $\eta = \min\{\gamma, 1 - \gamma\} \to \min\{1, \alpha\}/(\alpha + 1)$, which are the same as $k = \infty$. Hence, the regime lying between $k = 1 + 1/\alpha$ and $k = \infty$ should have the same scaling behaviors.

Taken together, we obtain

$$\gamma = \begin{cases} 0, & k < k^* \\ 1 - k^*/k, & k^* \le k < k^* + 1 \\ 1/(k^* + 1), & k \ge k^* + 1 \end{cases} \tag{S73}$$

$$\eta = \min\{\gamma, 1 - \gamma\} \tag{S74}$$

where $k^* = 1/\alpha$.

### S3.5 Connections with canonical ensembles

The piecewise function in our solutions raises an interesting question: What characterizes the discontinuous pattern at $k = k^*$ and $k = k^* + 1$? In this section, we establish a mapping between our model and a canonical ensemble system, showing that the observed critical points can be phenomenologically linked to phase transitions (Fig. S8).

For simplicity, we rescale this system through

$$\begin{aligned} K &= k - k^* \\ \Gamma &= k^*\gamma/(1 - \gamma) \end{aligned} \tag{S75}$$

$K = k - k^*$ and $\Gamma = k^*\gamma/(1-\gamma)$, obtaining

$$\Gamma = \begin{cases} \Gamma_a(K) \equiv 0, & K < 0 \\ \Gamma_b(K) \equiv K, & 0 \leq K < 1 \\ \Gamma_c(K) \equiv 1, & K \geq 1 \end{cases} \tag{S76}$$

Note that all smoothness conditions are preserved since the transformations in S75 are infinitely differentiable. Here we consider a system with three different states $a, b, c$ with corresponding energy density $E_a(h), E_b(h), E_c(h)$. Its partition function can be written as

$$Z = e^{-NE_a(h)} + e^{-NE_b(h)} + e^{-NE_c(h)} \tag{S77}$$

where $N$ is the total number of particles and $h$ is external field. We further assume that $E_a(h) = (2\epsilon h - 1)^2$, $E_b(h) = (2h-1)^2$, and $E_c(h) = [2\epsilon(1-h) - 1]^2$ where $\epsilon \to 0^+$. The introduction of $\epsilon$ is to distinguish state $a$ from state $c$, and we approximate this with limiting condition $E_a(h) = E_c(h) = 1$.

Next, we map $f \to (2\Gamma - 1)^2$, $N \to \ln n$, $h \to K$, and $E_i(h) = [2\Gamma_i(K) - 1]^2$. Hence, the two transition points $k^*$ and $k^* + 1$ corresponds to $h = 0$ and 1 in the canonical ensemble systems. To explore the nature of discontinuity at $k^*$ and $k^* + 1$, we now turn back to the analytical solutions of the mapped system.

Indeed, as $N \to \infty$, the free energy density $f = \ln Z/N$ tends to converge to the minimal energy $f = \min(E_a(h), E_b(h), E_c(h))$. Hence, the magnetization density $m = \frac{df}{dh}$ is noncontinuous at the boundary of two $E_i(h)$. In particular, the differences across the boundary is caused

by changes of base states, i.e. the mechanisms that dominate the current system. Therefore, there exists phase transitions at $h^*$ if $E_i(h^*) = E_j(h^*)$ for $i \neq j$. Hence, we obtain phase transition at $h^* = 0$ and $h^* = 1$ respectively. To sum up, we successfully recover the two transition points at $k^*$ and $k^* + 1$.

To unveil the origin of the transitions, here we inspect $u(z)$, defined as the number of attempts where a version of high score $x \to 1$ (i.e. potential $z \equiv 1 - x \to 0$) is retained. We can analytically derive its asymptotic distribution as

$$P_z(u) \sim \left\{ \frac{(1 - z^{1/k^*})[1 - z^{k/k^*}(1 - z)^k]}{1 - z^{1/k^*}(1 - z)} \right\}^{-Au} \sim [1 - z^{\min\{k/k^*, 1/k^*+1\}}]^{-Au} \tag{S78}$$

where $A$ is a constant independent of $z$ and $u$. Eq (5) enables us to calculate the expected life span of a high-quality version $\langle u(z) \rangle \sim \langle z^{-\min\{k/k^*, 1/k^*+1\}} \rangle$. The first critical point $k = k^*$ hence corresponds to the finiteness of this first moment $\langle u \rangle$. When $k$ is small ($k < k^*$), $\langle u \rangle$ is finite. In this region, although new versions build on past $k$ attempts, good versions will only be reused for a limited number of attempts. This is similar to an asymmetric (super-)*diffusive* random walk where the step size has finite expectation (renewal process), predicting a linear relationship between number of attempts and time cost. Once $k$ passes the critical threshold $k^*$, we find $\langle u \rangle = \infty$, hence a good version may be retained for an unlimited long period. This is similar to a *ballistic* random walk where the step size has infinite expectation, where the scaling behavior between steps (time cost) and distance (number of attempts) begins to emerge. The second phase transition originates from the competition between two dynamical forces: (a) the $k/k^*$ term represents the chance that the current best version gets forgotten due to $k$ consecutive attempts in creating new versions; (b) the $1/k^* + 1$ term captures the chance that the current best version is substituted by a

better one. Comparing the dominance of the two mechanisms points to the second transition point $k^* + 1$, beyond which $k$ plays no major role.

### S3.6 Functional forms of $\rho(x)$ and $p(x)$

Two important quantities in our model are $\rho(x)$, the score distribution for a new version, and $p(x)$, the probability to create a new version given reference score $x$. For simplicity we assume $\rho(x) \equiv 1$ and $p(x) = (1-x)^\alpha$ in main text. Here we show that similar results can be obtained as we consider a general class of functional forms of $\rho(x)$ and $p(x)$.

Indeed, since both quantities depend on the scoring system, we may fix one to a specific form. Consider two score systems $x$ and $y$ that can be derived through $y = c(x)$. We can derive the transformations as

$$\rho_X(x) = \rho_Y(c(x))c'(x) \tag{S79}$$

$$p_X(x) = p_Y(c(x)) \tag{S80}$$

Combining the two equations we find the quantities can be connected through

$$\rho_X/(p_Y^{-1} \circ p_X)' = \rho_Y \circ p_Y^{-1} \circ p_X \tag{S81}$$

Indeed, selecting appropriate transformations one can apply the derived protocols for other existing models in learning curve studies. To demonstrate this, let us consider a selection model documented in[42]. Here we define $\rho_X = x^{\beta-1}, \rho_Y = 1, p_X = 1$, we obtain $c(x) = x^\beta/\beta$ and $p_Y = 1$

(i.e. $\alpha = 0$), assuming $k = \infty$ we have

$$\langle x_n \rangle \sim \langle y_n^{*(1/\beta)} | k = \infty, \alpha = 0 \rangle \sim n^{-1/\beta} \tag{S82}$$

In this way we arrive at a system $y$ that is mathematically equivalent to existing model systems[42], where one has power law cost distribution, try new versions at every attempt and learns from all past experiences. Hence our approach is also able to recover this $n^{-1/\beta}$ scalings ($n^{-1/k}$ using notations in original paper[42]) documented in learning curve models through mathematical transformations. For following discussions we always assume $\rho \equiv 1$ and consider different forms of $p(x)$.

Our previous results have shown solutions for $p(x) = (1-x)^\alpha$, prompting us to consider a more general form using expansion

$$\ln(p(x^*) - p(1)) = \alpha \ln(1 - x^*) + o(\ln(1 - x^*)), \;\; x \to 1 \tag{S83}$$

where $\alpha \equiv \lim_{x^* \to 1} \frac{\ln p(x^*)}{\ln(1-x^*)} \geq 0$ captures the asymptomatic behavior of $p$ near $x^* \to 1$. If $p(1) > 0$, there is certain positive probability that one will create a new one, no matter how good she did, which will cause both $t_n$ and $x_n$ converging to positive limit. On the other hand, when $p(1) = 0$, we can approximate $p(x^*) \sim (1 - x^*)^\alpha$, hence we should observe the same scaling as $p(x^*) \sim (1 - x^*)^\alpha$. Indeed, all our previous derivations only rely on the power law tail of $x^{-k\alpha}$ rather than a precise power law form.

Despite its simplicity, the assumption enables us to work with a broad range of functions, including all functions that are analytic at $x^* = 1$ (e.g. $p = e^{c(1-x^*)} - 1 \sim c(1 - x^*)$) as well

as many that are not (e.g. $p = (1 - x^*)^c$ with non-integer $c$) through a single parameter $\alpha$. Note that this relaxation in the functional form of $p(x)$ is again closely related to the relaxation in $\rho(x)$ documented in[42] due to the relationship between the two quantities we discussed before.

### S3.7 Null models

Our model demonstrates that both experience and evaluations play an important role in dynamics of failure. To verify that both ingredients are necessary, we investigate two variants of the model.

To understand the role of experience, we explore a model (a) assuming that an individual does not reuse past versions. We find model (a) reduces to the case of $k = 0$, where each attempt is made independently. Again, we recover results from S3.2, predicting constant efficiency $t_n = 1$ and quality $x_n = 0.5$.

We then keep the experience mechanism, but eliminate the role of evaluations by assuming that one chooses to reuse past version regardless of its score. In other words, model (b) assumes that the probability to create a new version, $p$, is constant, independent of past scores. This allows us to write the master equation as

$$x^*_{n+1} \sim \begin{cases} U[0,1], & w.p.\ p \\ \delta(x^*_n), & w.p.\ 1-p \end{cases} \tag{S84}$$

By induction one has $x_n \sim U[0,1]$ for any $n$, again predicting constant efficiency $t_n = p$ and quality $x_n = 0.5$. This indicates that in the absence of evaluations the model fails to reproduce the observed scaling behavior. Indeed, the improvement in the original model is mainly driven by

reuse preference towards version with higher-scores, explaining why it does not exist in this null model.

Together, the predictions of these two alternative models indicate that a combination of the two ingredients is essential for the emergence of scaling observed in Fig. 4. One may also hypothesize that the uncovered patterns are affected if we define the finite capacity using the unit of time ($t$) rather than trials ($n$), prompting us to consider a model (c): Here we assume that individuals at time $t$ consider all past failures that occurred during a time window $\tau$, i.e. individuals at time $t$ consider all past failures that occurred during a time interval $(t-\tau, t]$, where the window size $\tau$, instead of our previous parameter $k$, measures how long one looks back upon past failures. We further assume that the number of components equals to one for simplicity. The previous master equation can be written as

$$x_n^* = \max_{t_m+\cdots+t_n \leq \tau} \{x_m\} \tag{S85}$$

$$x_n \sim \begin{cases} U[0,1], & w.p.\ (1-x_n^*)^\alpha \\ \delta(x_n^*), & w.p.\ 1-(1-x_n^*)^\alpha \end{cases} \tag{S86}$$

To solve this model, we note that the following equations hold.

$$|\{n_1 \leq n \leq n_2 : x_n = x_m^*\}| \leq n_2 - n_1 + 1 \tag{S87}$$

$$|\{n_1 \leq n \leq n_2 : x_n = x_m^*\}| \geq \sum_{i=0}^{[(n_2-n_1)/(\tau+1)]-1} \sum_{j=0}^{\tau} I(x_{n_1+(\tau+1)i+j} = x^*_{n_1+(\tau+1)i+i}) \geq [(n_2-n_1)/(\tau+1)] \tag{S88}$$

This is because, if we consider $\tau+1$ versions $(x_i, \cdots, x_{i+\tau})$, we should find (1) at least two of the versions are the same or (2) these are $\tau+1$ different versions. If (1) is true, i.e. $x_j = x_k$ for some

$i \le j < k \le i+\tau$, we have $x_j = x_k^*$, i.e. the duplicated version is a baseline version. Otherwise, (2) means that there are at least $\tau$ new versions, covering all versions over the last $\tau$ time units. Hence we have $x_{i+\tau+1}^* \in \{x_i, \cdots, x_{i+\tau}\}$.

Using the notations in previous derivations, we can also recover the master equation as

$$z_{m+1} = \begin{cases} z_m & w.p. \ \frac{[1-z_m^{\tau\alpha}(1-z_m)^\tau](1-z_m^\alpha)}{1-z_m^\alpha(1-z_m)} \sim O(1) \\ U[0, z_m] & w.p. \ \frac{[1-z_m^{\tau\alpha}(1-z_m)^\tau] z_m^{\alpha+1}}{1-z_m^\alpha(1-z_m)} \sim O(z_m^{\alpha+1}) \\ \min\{U_1[0,1], \cdots, U_\tau[0,1]\} & w.p. \ z_m^{\tau\alpha}(1-z_m)^\tau \sim O(z_m^{\tau\alpha}) \end{cases} \tag{S89}$$

To this end, we find that this variant is asymptotically similar to our original model, with $\tau^* = k^* = 1/\alpha$. Indeed, when a baseline version is out of date and gets replaced, the recency mechanism happens after $k^*$ ($\tau^*$) new versions have been created without reuse, explaining why $\tau^*$, the critical number of different versions to look back, equals to $k^*$, the critical number of versions to look back.

### S3.8 Failure streak length

To explain the fat-tailed distribution documented in Fig. 1, let us consider a single-component case of our model for simplicity. We assume that $q$, the probability for a new version to success, is independent of its score. We denote $N$ as the number of failures before success.

Assume $N \ge n$, i.e. one has not achieved success in the first $n$ attempts. For one to succeed in the $(n+1)$-th attempt, she needs to (1) create a new version at this time, corresponding to

probability $t_n \sim n^{-\gamma}$ and (2) succeed for this new version, which has probability $q$. Together we obtain

$$P(N = n | N \geq n) \sim q n^{-\gamma} \tag{S90}$$

Note that this form is closely related with Lindy's law[77,78]. Here the right hand side of the equation is decreasing, since a long failure streak indicates the existence of an (unsuccessful) version that has been used for a long period. Therefore, the same version is more likely reused again in the future, reducing the chance to create a new, successful version at the next step.

If we define the survival function $S(n) = P(N \geq n)$, this equation is equivalent to

$$1 - S(n+1)/S(n) \sim q n^{-\gamma} \tag{S91}$$

Using a continuous approximation we obtain

$$-\frac{dS}{S} \sim q n^{-\gamma} dn \tag{S92}$$

leading to the solution

$$P(N \geq n) = S(n) \sim e^{-cn^{1-\gamma}} \tag{S93}$$

Hence, it predicts that the length distribution follows the well-known Weibull distribution.

To further understand the Weibull form, here we point out that it is closely related to Heaps' law[73] caused by the reuse mechanism. Indeed, given that one needs to create $M$ different versions before success, the distribution can be formulated as an exponential model

$$P(M \geq m) = (1 - q)^m \tag{S94}$$

However, repeated reuse leads to a sub-linear scaling between $N$ and $M$, following the Heaps' law with exponent $1 - \gamma$:

$$M(N) = \sum_{n=1}^{N} t_n \sim \sum_{n=1}^{N} n^{-\gamma} \sim N^{1-\gamma} \tag{S95}$$

Combining the two equations one can obtain the same Weibull model

$$P(N \geq n) = S(n) \sim e^{-cn^{1-\gamma}} \tag{S96}$$

The completely random assumption is not necessary. Indeed, we can relax it by considering success probability $q$ as a function of evaluation score $x$. As long as (1) $q(x)$ is non-decreasing with $x$, hence a better score corresponds to a higher probability of success. (2) $q(x) < 1$ all $x$, characterizing an uncertain world where there is no guaranteed success. Now we have

$$P(M \geq m) = \left(1 - \int_0^1 q(x)dx\right)^m \tag{S97}$$

Using the sub-linear scaling between $M$ and $N$, the failure streak length is still captured by the Weibull distribution. An interesting insight from these results is that all quantities of interest exhibit scale-free properties. This means if we consider different criteria of success that are organized into hierarchal structures, our results are robust against the selection of criterion.

Another possibility that can lead to fat-tailed distributions is fitness heterogeneity[16]. Indeed, since different individuals may have different fitness, it might be possible that the fat tail of failure streaks can emerge without the reuse mechanism. To test if this is sufficient for modeling dynamics of failure, here we compare it with other observations, finding the fitness hypothesis cannot account for the observed patterns for a series of reasons:

1. Initial performance fails to predict eventual outcome. One direct prediction of the fitness hypothesis is the predictive power of initial performance for the eventual outcome. However, as shown in Figs. 4g-i, we find that for large $n$, the success and non-success group show no statistical differences at the first attempt, which is in strong contrast with our prediction.

2. Weak correlation between initial performance and failure streak. Assuming performance dynamics is mostly driven by fitness heterogeneity, those who succeeded with fewer failures should show better performance at the very beginning. Hence, one would expect a strong correlation between initial performance and failure streak. However, we find that across the three datasets, the correlation between the two is weak (Fig. S13a-c).

3. Fat tail remains as we control fitness. If the fat-tail is caused by a broad distribution of fitness, we should observe a narrower tail as we control the fitness through conditioning on initial performance. Our results show that, as we conditional on samples with top/bottom performance at the beginning, $P(N)$ still distinguishes from the exponential model (Fig. S13d-f).

4. Failure dynamics. Most importantly, the fitness hypothesis states that success and non-success groups lie on a continuous spectrum, hence we should not expect fundamental differences in their temporal patterns. To this end, it fails to account for the observed patterns documented in Figs. 4d-f.

## S4 Empirical measurements

### S4.1 Quantifying performance dynamics

Here we leverage our three datasets and compile three different measurements for performance.

For the NIH grant application dataset, we make use of the percentile scores assigned by NIH review panels. NIH uses a two-step peer review mechanism: Roughly half of the proposals are selected for the second round discussion, where each proposal is given a percentile score based on their percentile ranking among its peers. Percentile score has been widely used to measure the quality of R01 grant applications[27,79], reflecting judgment of expert reviewers. Although reviewers score are necessarily imperfect, there is growing evidence for strong correlations between percentile score and subsequent successes of the project[50,80]. One disadvantage of using the percentile score is that undiscussed proposals (those get rejected in the first round) do not have such scores. Moreover, since there exist differences concerning the discussion rate, applications lying on the boundary of discussion can have either marginal scores or no scores. Indeed, here we calculate the proportion of having a percentile score around 57% and plot the score distribution. We find as score exceeds 50, there are much fewer samples, since many proposals at this rank did not even get discussed and assigned a score (Fig. S4). To avoid discrimination across study sections, here we take score below 50 and regard the remaining proposals as undiscussed. We also vary the threshold to 55, finding results remain the same. Lower percentile scores indicate better performance. To be consistent with other measures (higher the better) we rescale the percentile scores using 1-0.01$\times$original score, so the values reported in main text are bigger the better.

To measure the performance in startup ventures, we leverage the investment amount in the first funding round as a proxy. Although there are a series of firm-level statistics that could potentially measure the quality of a venture, investment amount stands out as a preferred choice of representing investor evaluations. This definition does not account for geographical and industrial factors, as such information is not available to us, but it serves as a reasonable index of startup companies potentials in achieving their eventual goals (IPO or high-value M&As).

Similar to other frequently used measures in economics, investment amount follows a fat-tailed distribution and exhibits time-dependent properties. To address the two challenges, we take logarithmic of the investment amount and calculate z-score within each year. Denoting the amount of all investments made in year $t$ as $\{s_1^t, \cdots, s_n^t\}$, here we rescale the values into the performance score $z$ through

$$z_i^t = \frac{\log(s_i^t) - \mathrm{E}[\log(s^t)]}{\sqrt{\mathrm{Var}[\log(s^t)]}}$$

Once rescaled, we find $z_i^t$ approximately follow the standard normal distribution $N(0,1)$ independent from $t$, allowing us to directly compare attempts made in different years (Fig. S5a). We then compare first-round investment amounts for successful and failed attempts, finding the two samples are clearly separated (Fig. S5b).

Similarly, for terrorist attacks, one measure for performance is the number of individuals wounded. To this end, we collect wound statistics as our performance measure. As shown in Fig. S6b, fatal (successful) attacks also lead to a higher number of wounded individuals than others, validating the effectiveness of using wounded statistics as performance measurements. Re-

lated studies of terrorist attacks suggest the outcome of attacks follow a power law distribution (Fig. S6a), which is also confirmed in our dataset. To this end, we rescale the original values by $\log(wounded + 1)$ in our analysis.

### S4.2 Length distribution of failure streaks

The length distribution of the failure streak, defined as the number of failures before success, is measured directly from data and fitted using maximum likelihood estimation techniques [46]. We fit empirical data with discrete versions of exponential and Weibull (stretched exponential) forms using maximum likelihood estimation with parameters $x_{\min} = 2$. We compare the fitting results from alternative results, i.e. lognormal, power law, and truncated power law using likelihood ratio test[46], finding that Weibull distribution is consistently among the best functional forms (Table S2). To quantify the uncertainty of parameter estimations, we performed bootstrapping technique (100 times) to calculate optimal estimation for each round, and obtained standard error of parameter estimators. We also repeated the results for $x_{\min} = 3$, obtaining $\beta_1 = 0.596 \pm 0.032$, $\beta_2 = 0.540 \pm 0.175$, and $\beta_3 = 0.178 \pm 0.057$, which again statistically supports $\beta + \gamma = 1$.

### S4.3 Measuring failure dynamics

Given the highly skewed distributions of $N$ and $t_n$, to measure $T_n = t_n/t_1$ we first performed log transformation to calculate the mean and variance of $\log(T_n)$ from

$$\mathrm{E}[\log(T_n)] = \langle \log(t_n/t_1) \rangle \tag{S98}$$

$$\mathrm{Var}[\log(T_n)] = \langle[\log(t_n/t_1)]^2\rangle - \langle\log(t_n/t_1)\rangle^2 \quad \text{(S99)}$$

As the number of samples decreases dramatically with $n$, here we focus on $n \leq 10$ for $D_1$, $n \leq 7$ for $D_2$, and $n \leq 4$ for $D_3$.

The two equations immediately give us mean $\mathrm{E}[\log(T_n)]$ and standard error of the mean $\sqrt{\mathrm{Var}[\log(T_n)]/\text{sample size}}$, as plotted in Fig. 4. The divergence between the two groups can be detected as early as the second attempt. Although $T_1 \equiv 1$ by construction, Student's t-test rejects the hypothesis that $T_2$ between success and non-success groups are the same ($P = 0.000457$, 0.00773, and 0.0499, respectively).

To calculate the temporal scaling exponent $\gamma$, here we run linear regressions between $\log(n)$ and $\log(T_n)$ and take the negative slope as $\gamma$, i.e.

$$\log(t_n/t_1) = -\gamma \log(n) + c, \quad \text{(S100)}$$

yielding $\gamma_1 = 0.361 \pm 0.010$, $\gamma_2 = 0.509 \pm 0.036$ and $\gamma_3 = 0.668 \pm 0.143$ for success group, with $P < 0.001$ for all three datasets. We also performed individual fixed effect linear models using the same data, i.e.

$$\log(t_{n,j}) = -\gamma \log(n) + c_j + \epsilon_{n,j}, \quad \text{(S101)}$$

where $j$ is the index for different samples and $c_j$ is the fixed effect term for each agent $j$. We obtain similar results $\gamma_1 = 0.369 \pm 0.015$, $\gamma_2 = 0.408 \pm 0.054$ and $\gamma_3 = 0.414 \pm 0.171$. For non-success group there exists no significant relationships between $\log(n)$ and $\log(T_n)$ since the second failure (i.e. excluding $T_1$), with $P = 0.450$, $P = 0.884$ and $P = 0.823$ respectively. Together, these results offer strong empirical support for the diverging temporal patterns predicted by our model.

## S5 Prediction task

### S5.1 Predicting ultimate success

Our model uncovers time as an early signal for predicting eventual success and failure. This prediction is unexpected, since individuals through failures are aimed at improving their performance, rather than saving the time, hence we should expect the two groups have identical temporal patterns. To test this, we use $D_1$ to set up a simple prediction task (Fig. S10a). The goal of this task is not to design state-of-art classifiers for predicting success. Rather, to test the predictive power of temporal regularity. As such, our results offer a lower bound for the predictability of failure dynamics.

To this end, here we first assume a logistic classification model (Model 1) to predict the eventual success following $N$ consecutive failed attempts. For each $N$, we collect positive samples as individuals succeeded after $N$ failures versus negative samples as individuals dropped out after the same number of consecutive failures. Each sample has a $N-1$-dimensional predictor $t_n$ ($1 \leq n \leq N-1$). The classifier writes as

$$\frac{\log(success)}{1-\log(success)} = \beta_0 + \sum_{n=1}^{N-1} \beta_n \log(t_n) \tag{S102}$$

To evaluate the performance of our predictions, we calculate the AUC curve (average area under the receiver operating characteristic) over 10-fold cross validation for different $N$.

Our model further predicts that the inter-event time sequence follows a power law decay. If this is true, we should be able to further simplify the prediction model without losing a large frac-

tion of accuracy. Indeed, the power-law form means that we can rescale the $N-1$-dimensional feature $(\log(t_1), \cdots, \log(t_{n-1}))$ into two simple parameters by calculating the slope $-\gamma$ and intercept $\theta$ in the log-log plot, i.e.

$$\log(t_n) = -\gamma \log(n) + \theta \tag{S103}$$

Our prediction model 2 is based on the two variables $\gamma$ and $\theta$ to train a simpler classifier for eventual success, following

$$\frac{\log(success)}{1 - \log(success)} = \beta_0 + \beta_1\gamma + \beta_2\theta \tag{S104}$$

This simplification is expected to be inaccurate since it reduces a feature with high dimensions to data points into a 2-dimension feature. However, we surprisingly find that a similar prediction accuracy can be achieved as the previous model 1 across different $N$ (Fig. S10), accounting for more than 95% of accuracy in terms of additional predictive power (AUC-0.5).

Deeper studies in Model 2 offer additional evidence that is consistent with model predictions (Fig. S11). First, the coefficient for $\gamma$, $\beta_1$ remains positive (Fig. S11a), demonstrating that escalations in failures are related to eventual success. Our previous results also suggest that the membership of two groups are mainly determined by the learning process (different $k$) rather than the initial advantage (score/time at the first attempt). If so, we would expect the increasing majority of predictive power coming from information encoded in the parameter $\gamma$, especially for individuals with large $N$. To test this hypothesis, we apply an ad-hoc approach for variable importance in logistic regressions. We calculate the ratio coefficient for normalized input, i.e.

$$R = \frac{|\beta_1|[var(\gamma)]^{1/2}}{|\beta_2|[var(\theta)]^{1/2}} \tag{S105}$$

$R$ measures the ratio of coefficients once the two variables are normalized to have identical variance. We find that $R$ increases systematically with $n$ (Fig. S11b), concluding that the variable $\gamma$ contributes an increasing part of predictive powers as one fails more, supporting the hypothesis that the dynamic process itself, rather than the starting point, has larger impact on the eventual outcome following failures.

### S5.2 Testing power law model

Despite long history in using power law forms to model learning curves, the literature has also suggested other functional forms[49]. One of the frequently used alternatives is exponential function, predicting

$$t_n \sim ab^{-n} \tag{S106}$$

Indeed, recent studies have also suggested that the observed power law could be an artifact by average different samples and individuals should be characterized by an exponential decay[81].

The difficulty of testing different hypotheses in our datasets comes from small sample sizes: in contrast to industrial production or simple individual tasks, it is almost impossible to observe large number of failures from a single individual. Hence directly comparing the fitting of different models would suffer from overfitting issues. To this end, here for each individual sample, we take all but last one inter-event time for model fitting, comparing model predictions for the last inter-event time. This out-of-sample testing technique helps to rule out the possibility of overfitting.

Using this method we compare the performance of power law, exponential and linear models

in characterizing $t_n$ for each individual, measuring their prediction error (Fig. S9). We find that across the three datasets, the power law model yields minimum error in more cases.

## S6 Robustness checks

### S6.1 Definition of successes and failures

We vary our definition of successes and failures across different datasets. For $D_1$ we remove all renewal/resubmission successes and only focus on new applications, finding our results are not dominated by resubmissions(Fig. S21). For $D_2$ we vary the definition of success for a startup. Previously we have considered IPO and high-value M&A as success. Similar with hit papers defined in science of science, we define high-value M&As as those with transaction value ranking top 1% among all transactions in the same year. We vary this definition to top 5% transactions (Fig. S24) or exclude all M&As (Fig. S25), finding our conclusions still hold. For $D_3$ we also tried restricting attack types to be aimed at human beings (Fig. S26), including assassinations, bombing/explosions and assaults, which also yield similar results.

### S6.2 Threshold for being inactive in the system

The definition of non-success group depends on the threshold for inactive in the system. In main text we set up the threshold as 5 years, i.e. if one does not appear in the system for the last 5 years, we consider she as drop-out samples. To test the effect of this threshold, here we repeat our main results for 2 years (Figs. S14,S16,S18) and 8 years (Figs. S15,S17,S19), respectively. We find all

our results are robust as we tune this criterion.

### S6.3 Comparing first failures versus halfway/penultimate failures

Figure 4 showed the performance divergence patterns in two groups using first and second failures. Here we also compares the first failures versus halfway failures or penultimate failures, finding the same patterns exist (Fig. S28).

### S6.4 Other checks

For $D_1$ we further confirmed that only focusing on failures before the first success yield similar results. Indeed, as we further plot $T_n$ for samples with and without prior success, we find the dynamical patterns remain the same (Fig. S20). Lastly, we check the threshold of discussion score, considering original percentile score higher 55, rather than 50, as undiscussed. All these variants show results consistent with Fig. 1 and Fig. 4 (Fig. S23).

For $D_3$ we also check our definition of terrorist organizations. To this end, we downloaded additional information from GTD website, obtaining a filtered list of perpetrator groups. We find our results remain similar as we limit our analysis within groups on the list (Fig. S27).

1. Fortunato, S. *et al.* Science of science. *Science* **359**, eaao0185 (2018).

2. Azoulay, P. *et al.* Toward a more scientific science. *Science* **361**, 1194–1197 (2018).

3. Harford, T. *Adapt: Why success always starts with failure* (Farrar, Straus and Giroux, 2011).

4. Fleming, L. Recombinant uncertainty in technological search. *Management science* **47**, 117–132 (2001).

5. Wuchty, S., Jones, B. F. & Uzzi, B. The increasing dominance of teams in production of knowledge. *Science* **316**, 1036–1039 (2007).

6. Jones, B. F. The burden of knowledge and the death of the renaissance man: Is innovation getting harder? *The Review of Economic Studies* **76**, 283–317 (2009).

7. Petersen, A. M., Riccaboni, M., Stanley, H. E. & Pammolli, F. Persistence and uncertainty in the academic career. *Proceedings of the National Academy of Sciences* **109**, 5213–5218 (2012).

8. Clauset, A., Arbesman, S. & Larremore, D. B. Systematic inequality and hierarchy in faculty hiring networks. *Science advances* **1**, e1400005 (2015).

9. Sinatra, R., Wang, D., Deville, P., Song, C. & Barabási, A.-L. Quantifying the evolution of individual scientific impact. *Science* **354**, aaf5239 (2016).

10. Liu, L. *et al.* Hot streaks in artistic, cultural, and scientific careers. *Nature* **559**, 396 (2018).

11. Jara-Figueroa, C., Jun, B., Glaeser, E. L. & Hidalgo, C. A. The role of industry-specific, occupation-specific, and location-specific knowledge in the growth and survival of new firms. *Proceedings of the National Academy of Sciences* **115**, 12646–12653 (2018).

12. Hidalgo, C. *Why information grows: The evolution of order, from atoms to economies* (Basic Books, 2015).

13. Barabasi, A.-L. The origin of bursts and heavy tails in human dynamics. *Nature* **435**, 207–211 (2005).

14. Gonzalez, M. C., Hidalgo, C. A. & Barabasi, A.-L. Understanding individual human mobility patterns. *Nature* **453**, 779–782 (2008).

15. Brockmann, D., Hufnagel, L. & Geisel, T. The scaling laws of human travel. *Nature* **439**, 462–465 (2006).

16. Castellano, C., Fortunato, S. & Loreto, V. Statistical physics of social dynamics. *Reviews of modern physics* **81**, 591 (2009).

17. Malmgren, R. D., Stouffer, D. B., Campanharo, A. S. & Amaral, L. A. N. On universality in human correspondence activity. *Science* **325**, 1696–1700 (2009).

18. Argote, L. & Epple, D. Learning curves in manufacturing. *Science* **247**, 920 (1990).

19. Sitkin, S. B. Learning through failure: the strategy of small losses. *Research in organizational behavior* **14**, 231–266 (1992).

20. Yelle, L. E. The learning curve: Historical review and comprehensive survey. *Decision sciences* **10**, 302–328 (1979).

21. Dutton, J. M. & Thomas, A. Treating progress functions as a managerial opportunity. *Academy of management review* **9**, 235–247 (1984).

22. Shrager, J., Hogg, T. & Huberman, B. A. A graph-dynamic model of the power law of practice and the problem-solving fan-effect. *Science* **242**, 414–416 (1988).

23. Levitt, B. & March, J. G. Organizational learning. *Annual review of sociology* **14**, 319–338 (1988).

24. Huber, G. P. Organizational learning: The contributing processes and the literatures. *Organization science* **2**, 88–115 (1991).

25. Edmondson, A. Psychological safety and learning behavior in work teams. *Administrative science quarterly* **44**, 350–383 (1999).

26. Gross, C. P., Anderson, G. F. & Powe, N. R. The relation between funding by the national institutes of health and the burden of disease. *New England Journal of Medicine* **340**, 1881–1887 (1999).

27. Ginther, D. K. *et al.* Race, ethnicity, and nih research awards. *Science* **333**, 1015–1019 (2011).

28. Li, D. & Agha, L. Big names or big ideas: Do peer-review panels select the best science proposals? *Science* **348**, 434–438 (2015).

29. Kaplan, S. N. & Lerner, J. Venture capital data: Opportunities and challenges. In *Measuring Entrepreneurial Businesses: Current Knowledge and Challenges* (University of Chicago Press, 2016).

30. Eggers, J. & Song, L. Dealing with failure: Serial entrepreneurs and the costs of changing industries between ventures. *Academy of Management Journal* **58**, 1785–1803 (2015).

31. Gompers, P., Kovner, A., Lerner, J. & Scharfstein, D. Performance persistence in entrepreneurship. *Journal of Financial Economics* **96**, 18–32 (2010).

32. National Consortium for the Study of Terrorism and Responses to Terrorism (START). *Global Terrorism Database [Data file]* (2018).

33. Clauset, A. & Gleditsch, K. S. The developmental dynamics of terrorist organizations. *PloS one* **7**, e48633 (2012).

34. Johnson, N. *et al.* Pattern in escalations in insurgent and terrorist activity. *Science* **333**, 81–84 (2011).

35. Durrett, R. *Probability: theory and examples* (Cambridge university press, 2010).

36. Bass, R. F. *Stochastic processes*, vol. 33 (Cambridge University Press, 2011).

37. Argote, L. *Organizational learning: Creating, retaining and transferring knowledge* (Springer Science & Business Media, 2012).

38. Dahlin, K. B., Chuang, Y.-T. & Roulet, T. J. Opportunity, motivation, and ability to learn from failures and errors: Review, synthesis, and ways to move forward. *Academy of Management Annals* **12**, 252–277 (2018).

39. Levy, F. K. Adaptation in the production process. *Management Science* **11**, B–136 (1965).

40. Newell, A. & Rosenbloom, P. S. Mechanisms of skill acquisition and the law of practice. *Cognitive skills and their acquisition* **1**, 1–55 (1981).

41. Anderson, J. R. Acquisition of cognitive skill. *Psychological review* **89**, 369 (1982).

42. Muth, J. F. Search theory and the manufacturing progress function. *Management Science* **32**, 948–962 (1986).

43. McNerney, J., Farmer, J. D., Redner, S. & Trancik, J. E. Role of design complexity in technology improvement. *Proceedings of the National Academy of Sciences* **108**, 9008–9013 (2011).

44. Wright, T. P. Factors affecting the cost of airplanes. *Journal of the aeronautical sciences* **3**, 122–128 (1936).

45. Snoddy, G. S. Learning and stability: a psychophysiological analysis of a case of motor learning with clinical applications. *Journal of Applied Psychology* **10**, 1 (1926).

46. Clauset, A., Shalizi, C. R. & Newman, M. E. Power-law distributions in empirical data. *SIAM review* **51**, 661–703 (2009).

47. Barabási, A.-L. & Albert, R. Emergence of scaling in random networks. *Science* **286**, 509–512 (1999).

48. Bettencourt, L. M., Lobo, J., Helbing, D., Kühnert, C. & West, G. B. Growth, innovation, scaling, and the pace of life in cities. *Proceedings of the national academy of sciences* **104**, 7301–7306 (2007).

49. Ritter, F. E. & Schooler, L. J. The learning curve. *International encyclopedia of the social and behavioral sciences* **13**, 8602–8605 (2001).

50. Stephan, P. E. *How economics shapes science*, vol. 1 (Harvard University Press Cambridge, MA, 2012).

51. Paik, Y. Serial entrepreneurs and venture survival: Evidence from us venture-capital-financed semiconductor firms. *Strategic Entrepreneurship Journal* **8**, 254–268 (2014).

52. Walsh, G. S., Cunningham, J. A. *et al.* Business failure and entrepreneurship: emergence, evolution and future research. *Foundations and Trends® in Entrepreneurship* **12**, 163–285 (2016).

53. McGrath, R. G. Falling forward: Real options reasoning and entrepreneurial failure. *Academy of Management review* **24**, 13–30 (1999).

54. Edmondson, A. C. Strategies for learning from failure. *Harvard business review* **89**, 48–55 (2011).

55. Shepherd, D. A. Learning from business failure: Propositions of grief recovery for the self-employed. *Academy of management Review* **28**, 318–328 (2003).

56. Denrell, J. Vicarious learning, undersampling of failure, and the myths of management. *Organization Science* **14**, 227–243 (2003).

57. Kim, J.-Y. & Miner, A. S. Vicarious learning from the failures and near-failures of others: Evidence from the us commercial banking industry. *Academy of Management Journal* **50**, 687–714 (2007).

58. Edmondson, A. C. Learning from mistakes is easier said than done: Group and organizational influences on the detection and correction of human error. *The Journal of Applied Behavioral Science* **40**, 66–90 (2004).

59. Madsen, P. M. These lives will not be lost in vain: Organizational learning from disaster in us coal mining. *Organization Science* **20**, 861–875 (2009).

60. Baum, J. A. & Dahlin, K. B. Aspiration performance and railroads patterns of learning from train wrecks and crashes. *Organization Science* **18**, 368–385 (2007).

61. Haunschild, P. R. & Sullivan, B. N. Learning from complexity: Effects of prior accidents and incidents on airlines' learning. *Administrative science quarterly* **47**, 609–643 (2002).

62. Madsen, P. M. & Desai, V. Failing to learn? The effects of failure and success on organizational learning in the global orbital launch vehicle industry. *Academy of Management Journal* **53**, 451–476 (2010).

63. Sahal, D. A theory of progress functions. *AIIE Transactions* **11**, 23–29 (1979).

64. Roberts, P. A theory of the learning process. *Journal of the Operational Research Society* **34**, 71–79 (1983).

65. Kluger, A. N. & DeNisi, A. The effects of feedback interventions on performance: A historical review, a meta-analysis, and a preliminary feedback intervention theory. *Psychological bulletin* **119**, 254 (1996).

66. Asher, H. *Cost-quantity relationships in the airframe industry*. Ph.D. thesis, The Ohio State University (1956).

67. Crossman, E. A theory of the acqusition of speed-skill. *Ergonomics* **2**, 153–166 (1959).

68. Kauffman, S. & Levin, S. Towards a general theory of adaptive walks on rugged landscapes. *Journal of theoretical Biology* **128**, 11–45 (1987).

69. Levinthal, D. A. Adaptation on rugged landscapes. *Management science* **43**, 934–950 (1997).

70. Denrell, J. & March, J. G. Adaptation as information restriction: The hot stove effect. *Organization Science* **12**, 523–538 (2001).

71. Laird, J., Rosenbloom, P. & Newell, A. *Universal subgoaling and chunking: The automatic generation and learning of goal hierarchies*, vol. 11 (Springer Science & Business Media, 2012).

72. Loreto, V., Servedio, V. D., Strogatz, S. H. & Tria, F. Dynamics on expanding spaces: modeling the emergence of novelties. In *Creativity and universality in language*, 59–83 (Springer, 2016).

73. Heaps, H. S. *Information retrieval, computational and theoretical aspects* (Academic Press, 1978).

74. Simon, H. A. On a class of skew distribution functions. *Biometrika* **42**, 425–440 (1955).

75. Tria, F., Loreto, V., Servedio, V. D. P. & Strogatz, S. H. The dynamics of correlated novelties. *Scientific reports* **4**, 5890 (2014).

76. Iacopini, I., Milojević, S. & Latora, V. Network dynamics of innovation processes. *Physical review letters* **120**, 048301 (2018).

77. Mandelbrot, B. B. *The fractal geometry of nature*, vol. 1 (WH freeman New York, 1982).

78. Taleb, N. N. *The black swan: The impact of the highly improbable*, vol. 2 (Random house, 2007).

79. Jacob, B. A. & Lefgren, L. The impact of research grant funding on scientific productivity. *Journal of public economics* **95**, 1168–1177 (2011).

80. Li, D., Azoulay, P. & Sampat, B. N. The applied value of public investments in biomedical research. *Science* **356**, 78–81 (2017).

81. Heathcote, A., Brown, S. & Mewhort, D. The power law repealed: The case for an exponential law of practice. *Psychonomic bulletin & review* **7**, 185–207 (2000).

| Category | Reference | Time | Performance | Power law | Coexistence |
|---|---|---|---|---|---|
| Adaptation | Crossman[67] | ✓ | ✗ | ✗ | ✗ |
| | Kauffman & Levin[68] | ✗ | ✓ | ✗ | ✗ |
| | Denrell & March[70] | ✗ | ✓ | ✗ | ✗ |
| Search | Roberts[64] | ✗ | ✓ | ✓ | ✗ |
| | Muth[42] | ✗ | ✓ | ✓ | ✗ |
| | Mcnerney *et al*[43] | ✗ | ✓ | ✓ | ✗ |
| Individual learning | Newell *et al*[40] | ✓ | ✗ | ✓ | ✗ |
| | Anderson[41] | ✓ | ✗ | ✓ | ✗ |
| Urn | Simon[74] | ✗ | ✗ | ✓ | ✗ |
| | Tria *et al*[75] | ✓ | ✗ | ✓ | ✓ |
| | Iacopini *et al*[76] | ✓ | ✗ | ✓ | ✓ |
| Other | Levy[39] | ✗ | ✓ | ✗ | ✗ |
| | Shrager *et al*[22] | ✗ | ✓ | ✗ | ✗ |
| | Sahal[63] | ✓ | ✗ | ✓ | ✗ |
| | Johnson *et al*[34] | ✓ | ✓ | ✓ | ✗ |
| | Clauset & Gleditsch[33] | ✓ | ✓ | ✓ | ✗ |

Table S1: **Literature review of relevant models.** We test whether the models listed can predict (1) Time: time reduction; (2) Performance: performance improvement (or reduction in any cost other than time); (3) Power law: analytical form of power law scaling; (4) Coexistence: coexistence of two groups with different dynamics (success and non-success groups in this paper). We find that none of the existing models can predict all the observations in our paper.

| | Exponential | Lognormal | Power law | Truncated power law |
|---|---|---|---|---|
| NIH grants | *** | N.S. | *** | *** |
| Startups | *** | N.S. | *** | N.S. |
| Terrorist attacks | *** | N.S. | N.S. | N.S. |

Table S2: Comparing different functional forms of distributions with Weibull distributions. All significant terms denote the degree that Weibull distribution is preferred over the other. Among all alternatives, only lognormal models show comparable fitting performance. Yet lognormal model uses two free parameters while the shape parameter of Weibull distribution is constrained by the scaling identity (Eq. 4 in main text). ***: $p < 0.01$, N.S.: $p > 0.1$.

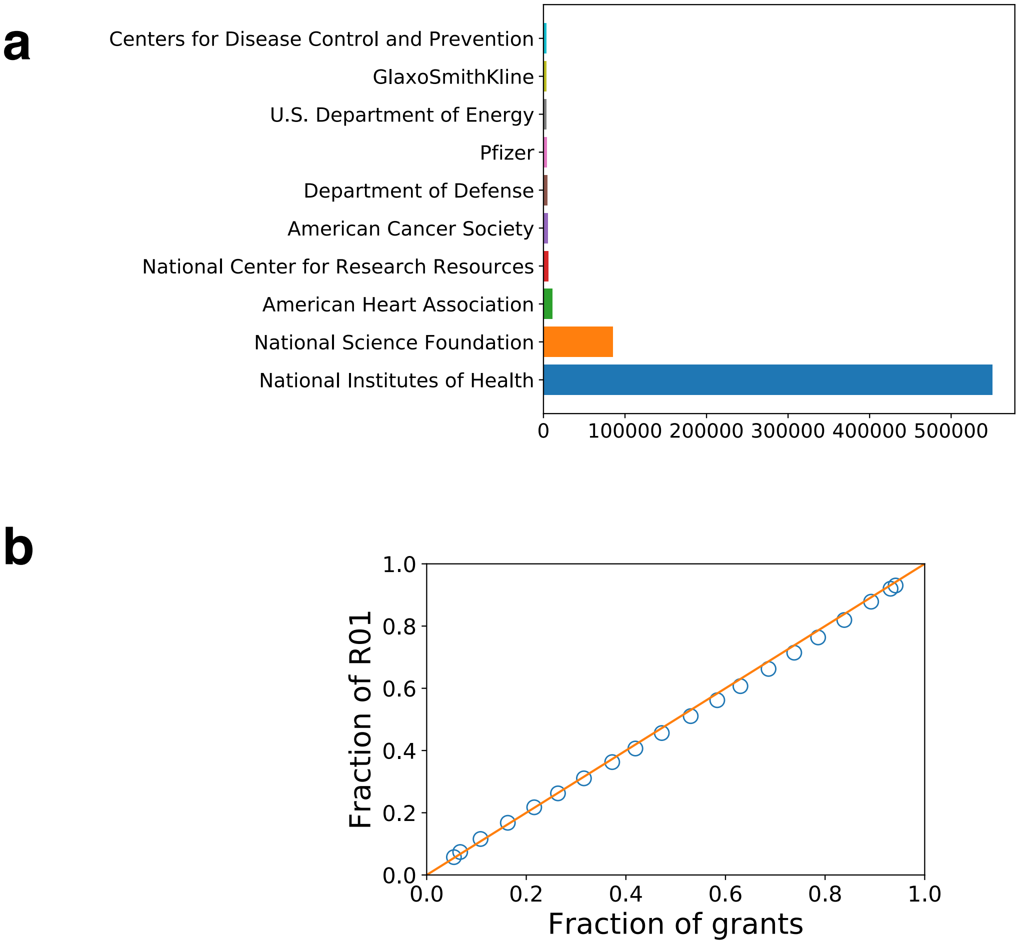


Figure S1: **Data coverage test for $D_1$.** (a) Coverage of NIH grants in biomedical research, according to WOS acknowledgment data. NIH represents the majority of funding sources (81% out of top 10 agencies). (b) Fraction of all grants versus R01 grants through individual careers are almost the same. Hence R01 grant application data represents as an unbiased sampling of the NIH landscape.

**a**

**b**

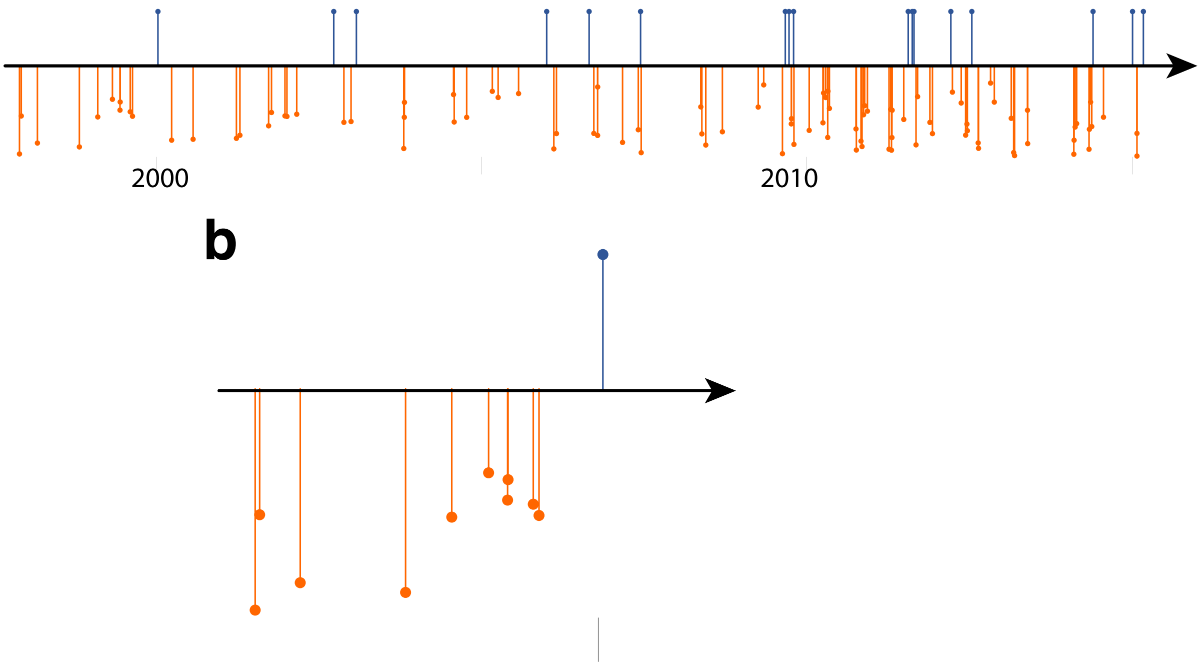


Figure S2: **Time series of R01 applications in NIH grant systems.** (a) Visualization of one scientist's application history Orange lines show failed applications, while blue lines show succeeded applications. Length of orange lines show NIH evaluation scores, shorter lines correspond to better performance as evaluated by review panels. (b) Subsequence in (a) of all attempts until the first success. Some applications do not have precise submission date, particularly those submitted before 2001, but their submission time can be inferred from proposed project end date of each application. For grants submitted after 2001, we compared the inferred and actual submission date, finding nearly perfect consistency between the two (Pearson correlation $r = 0.98$).

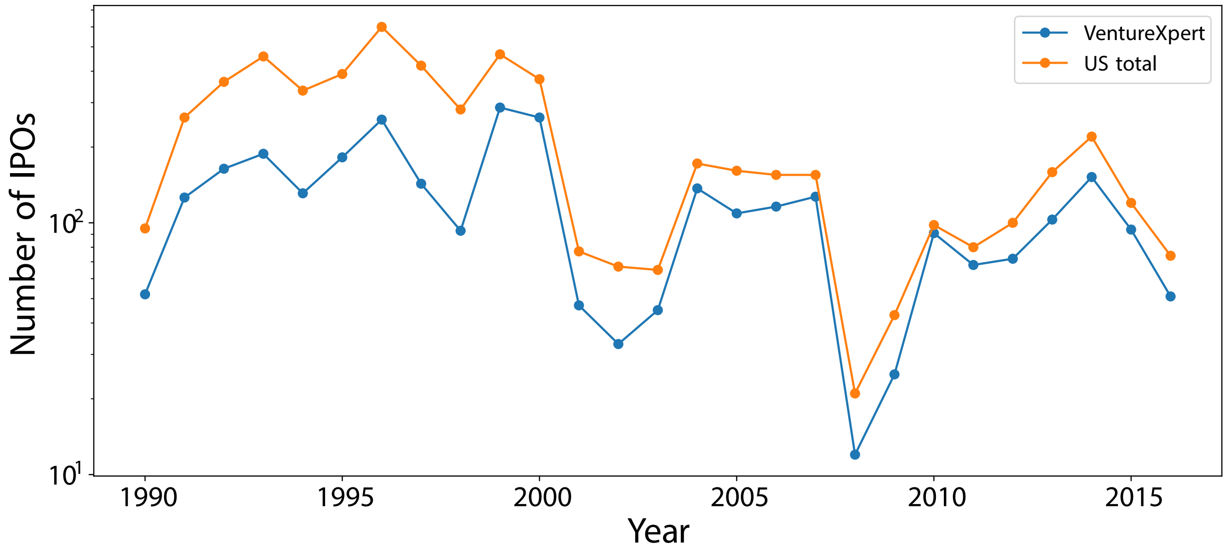


Figure S3: **Data coverage test for $D_2$.** Comparison of IPOs recorded in VentureXpert versus US market total. Our dataset captures a significant fractions of IPOs, with the ratio between the two statistics remaining stable across time, indicating our data source represents as an unbiased sampling of the whole US market.

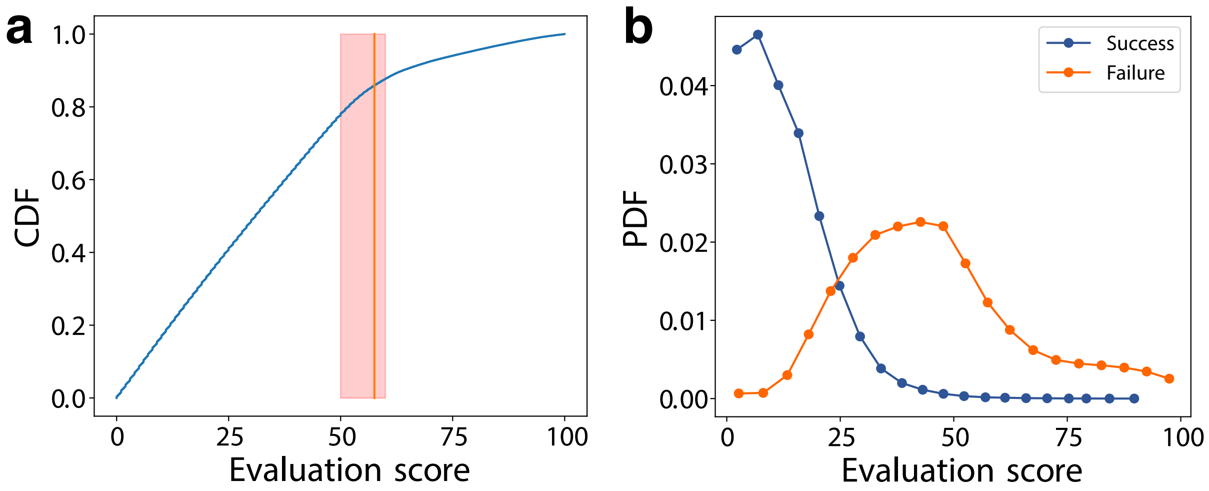


Figure S4: **Distribution of evaluation score for $D_1$.** (a) We find the distribution of evaluation score is uniform between $[0, 50]$, but begins to truncate between $[50, 60]$, where the probability of getting a score lies around $57\%$. (b) Here we measure the evaluation scores for successful and failed attempts, finding the distributions are well separated.

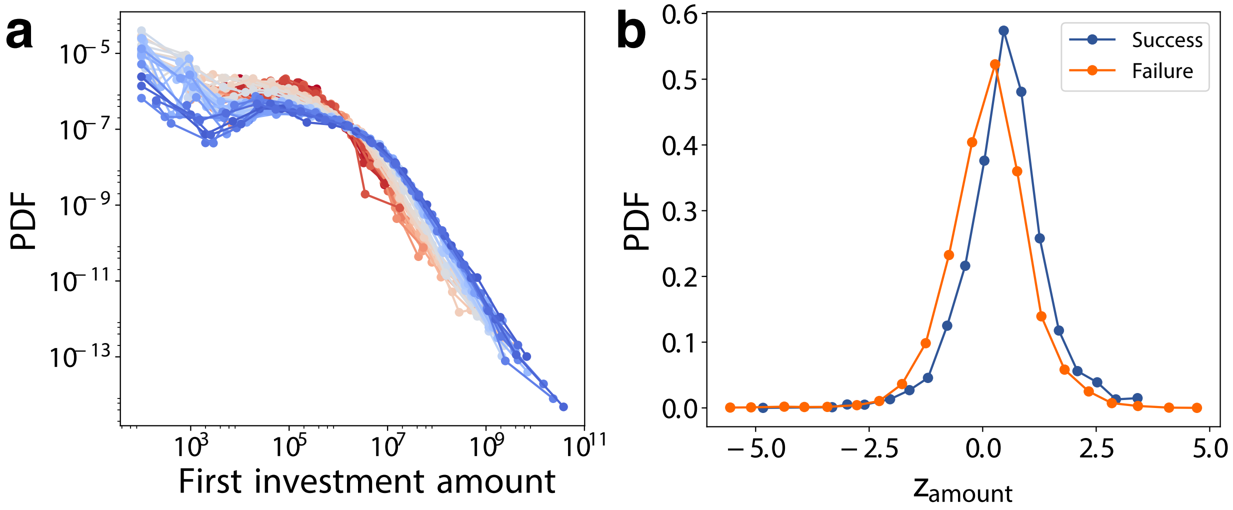


Figure S5: **Distribution of first investment amount for $D_2$.** (a) The amount of first investment follows a fat-tailed distribution and increases with year, prompting us to compare amount within year to account for such growth. (b) Here we measure the first investment amount for successful and failed attempts, finding the distributions are well separated. To account for fat tails and temporal changes we use z-score of $\log(amount)$ within a year.

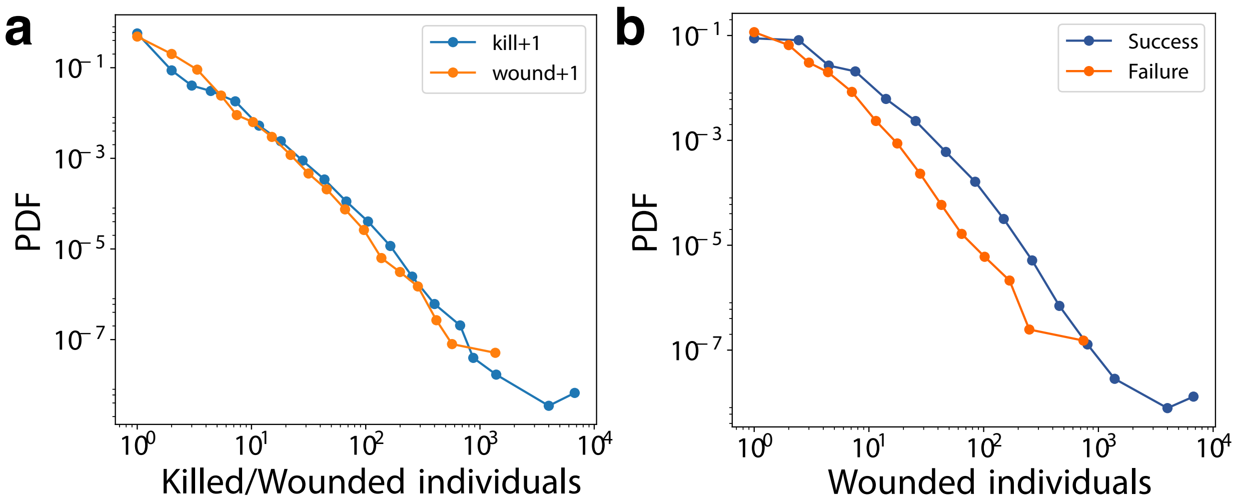


Figure S6: **Distribution of killed and wounded individuals for $D_3$.** (a) The number of killed and wounded individuals follow power law distributions, prompting us to take $\log(wounded + 1)$ as our performance measure. (b) Here we measure the number of wounded individuals for successful and failed attempts, finding the distributions are well separated.

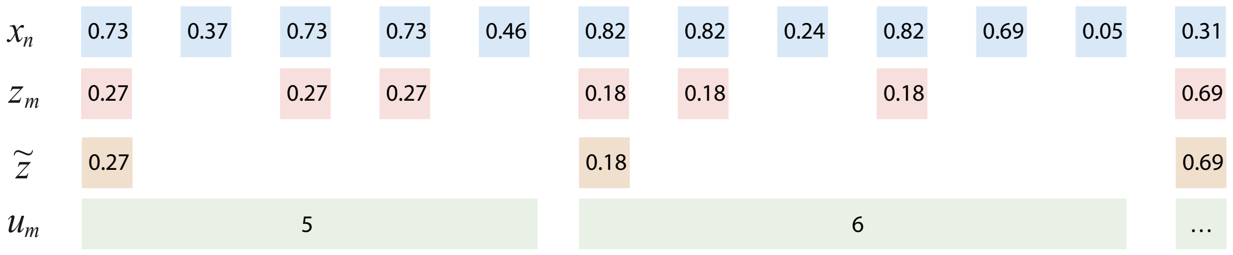


Figure S7: **Illustration of model solutions.** Here we visualize the notations used for solving the model. $x_n$ denotes the score for the $n$-th attempt, $z_m \equiv 1 - x_n$ corresponds to the potential given the best scoring among past $k$ failures. $\tilde{z}$ consists of all different $z_m$ as they first appear. $u$ measures the distance between two $\tilde{z}$-s, following a power law distribution as derived.

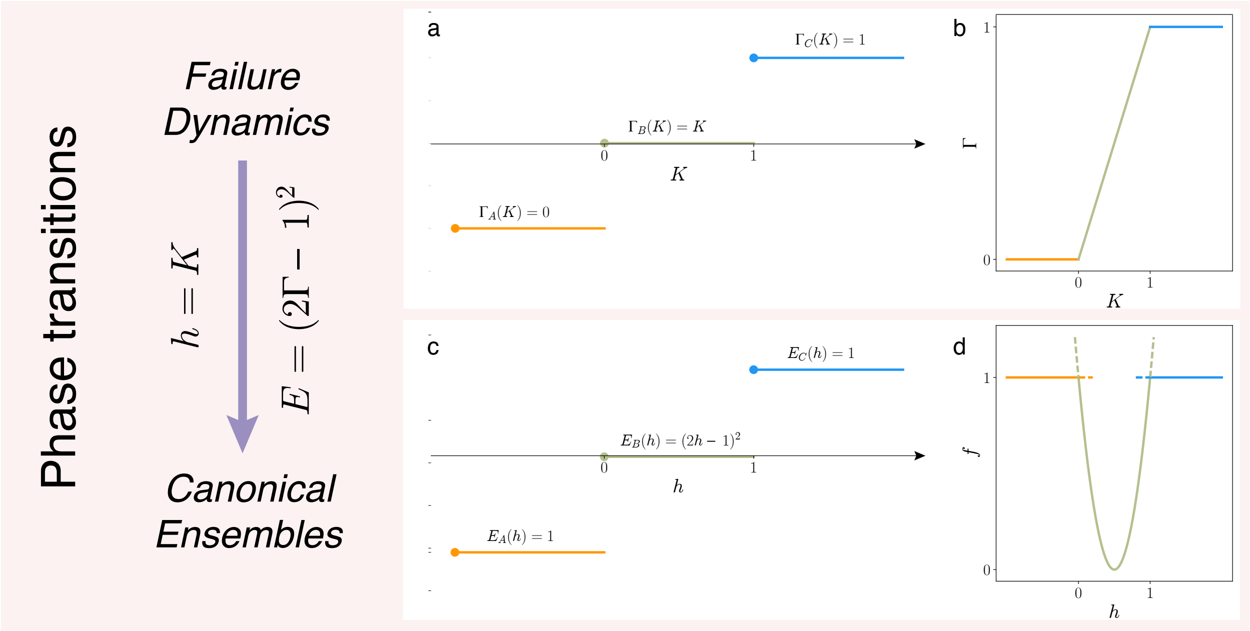


Figure S8: **Illustration of mapping between failure dynamics (a,b) and canonical ensembles (c,d)**. The canonical system is characterized by three different states $a, b, c$ with corresponding energy density $E_a(h), E_b(h), E_c(h)$. We further assume that $E_a(h) = (2\epsilon h - 1)^2$, $E_b(h) = h - h^2$, and $E_c(h) = [2\epsilon(1 - h) - 1]^2$ where $\epsilon \to 0^+$. The introduction of $\epsilon$ is to distinguish state $a$ from state $c$, and we approximate this with limiting condition $E_a(h) = E_c(h) = 0$. We map $f \to (2\Gamma - 1)^2$, $N \to \ln n$, $h \to K$, and $E_i(h) = [2\Gamma_i(K) - 1]^2$. Hence, the two transition points $k^*$ and $k^* + 1$ corresponds to $h = 0$ and 1 in the canonical ensemble systems.

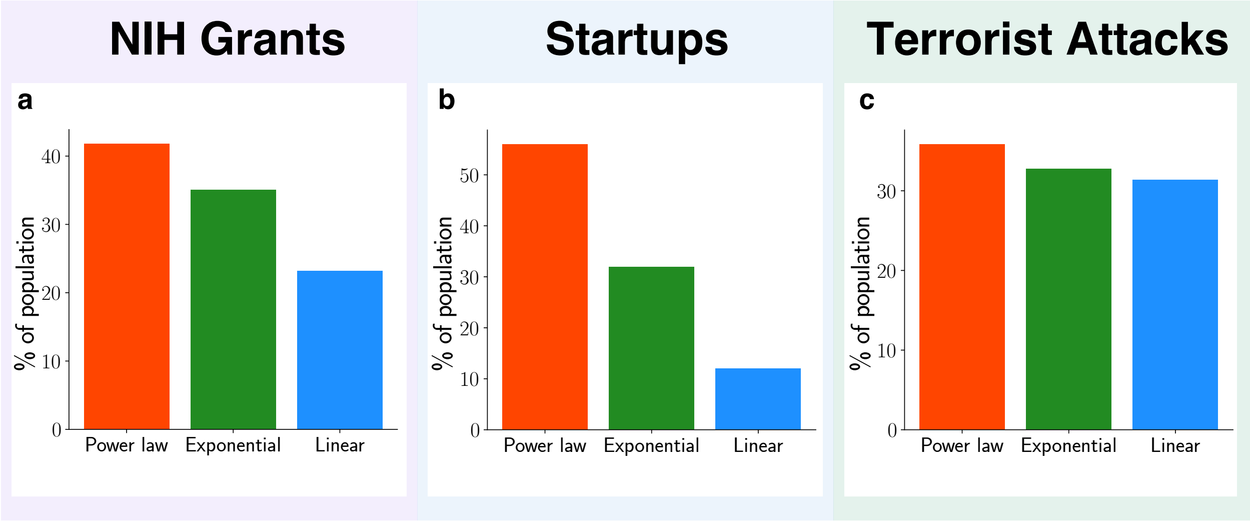


Figure S9: **Comparison of different models of temporal dynamics.** We calculate the frequency that each model reaches minimum error among all three forms. Power law model offers consistently better predictions.

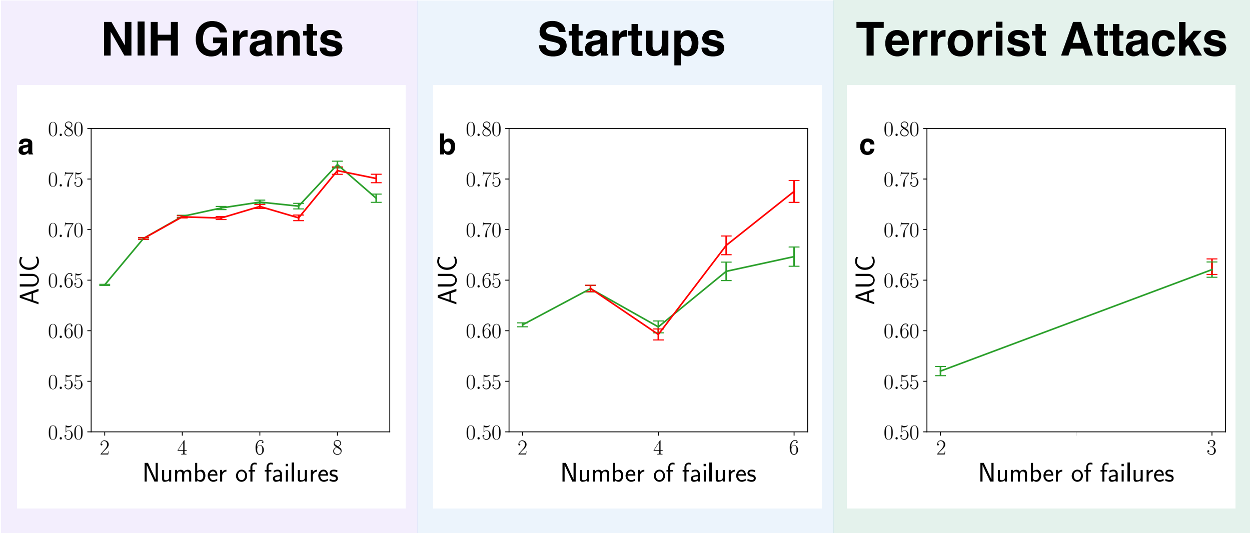


Figure S10: **Area Under the curve of the Receiver Operating Characteristic (AUROC) across three datasets**. Green lines denote results from prediction model 1, red lines denote results from prediction model 2. Values are obtained from 10-fold cross validation across 50 randomized iterations.

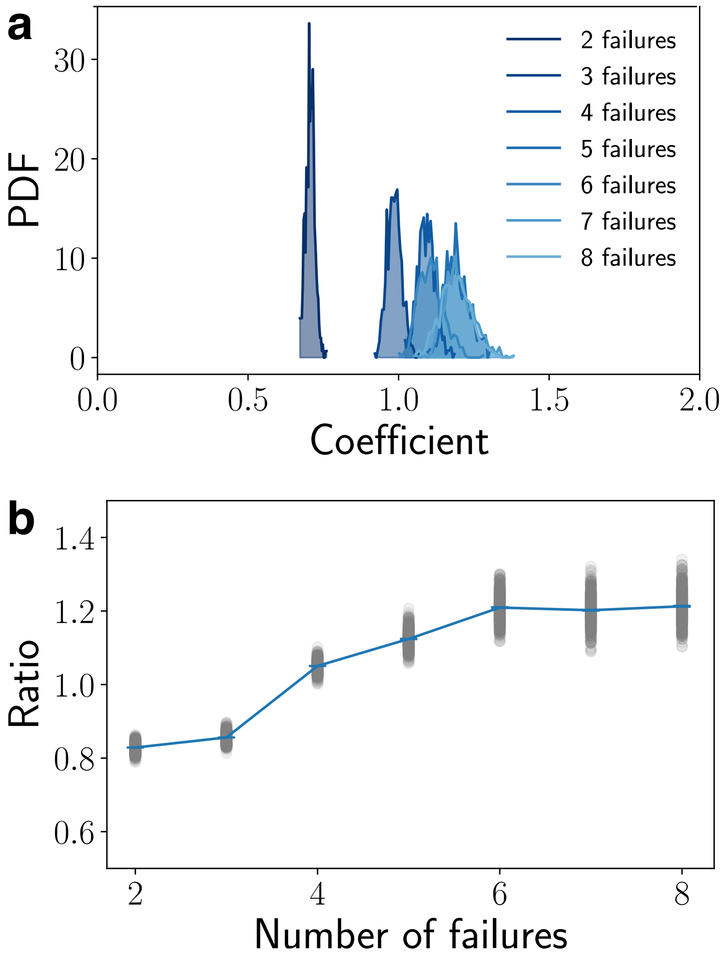


Figure S11: **Analysis of prediction task.** (a) Distribution of coefficient $\beta_1$ from prediction model 2 from $D_1$. We find that consistent with model predictions, $\beta_1$ is positive across different $N$. (b) Variance importance ratio for prediction task on $D_1$. Calculating variance importance ratio $R$ for our prediction model 2, we find an increasing proportion of uncovered predictive power contributed by $\gamma$, the slope of power law scaling.

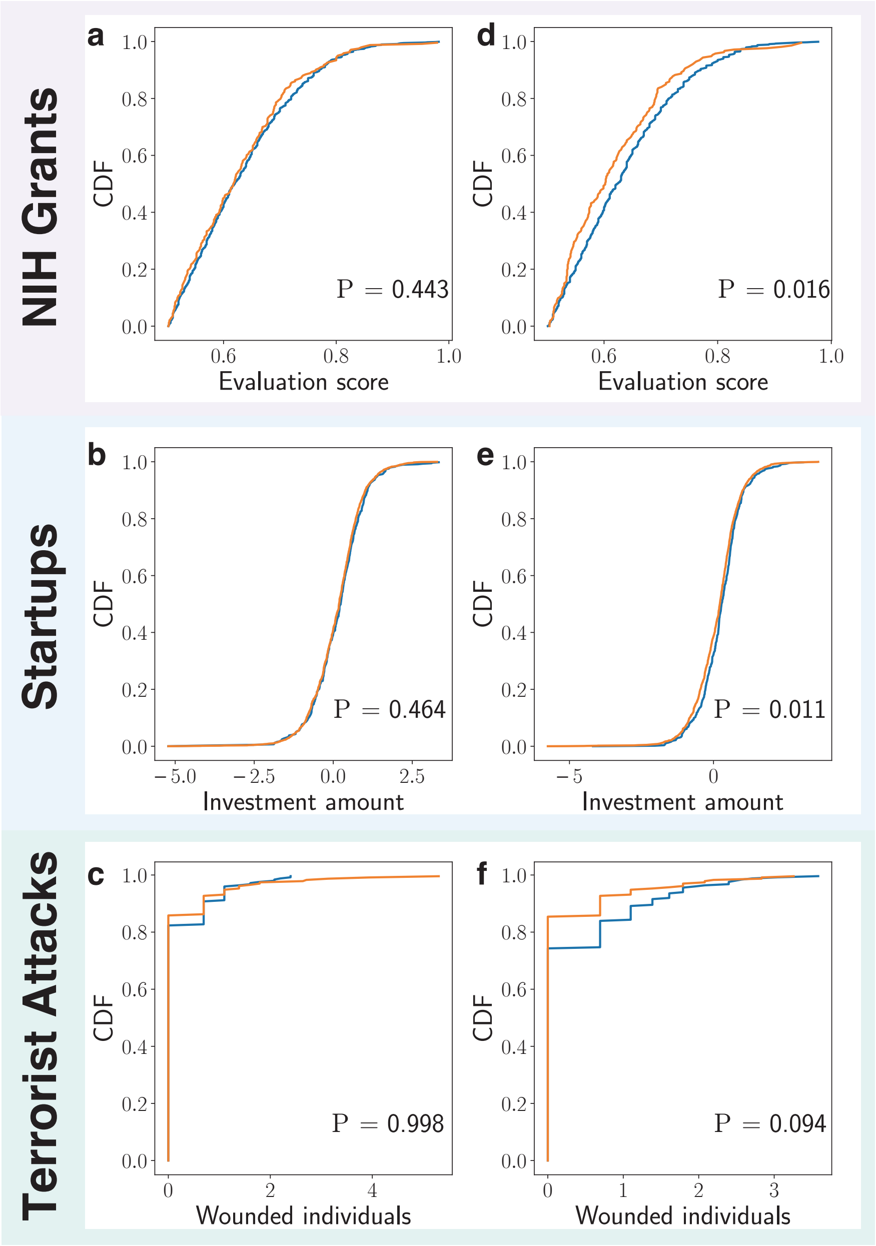


Figure S12: **Performance dynamics of failure**. Here we test performance dynamics using KS test. a-c show no significant differences for success and non-success group at the first attempt, while d-f show they are well separated at the second attempt.

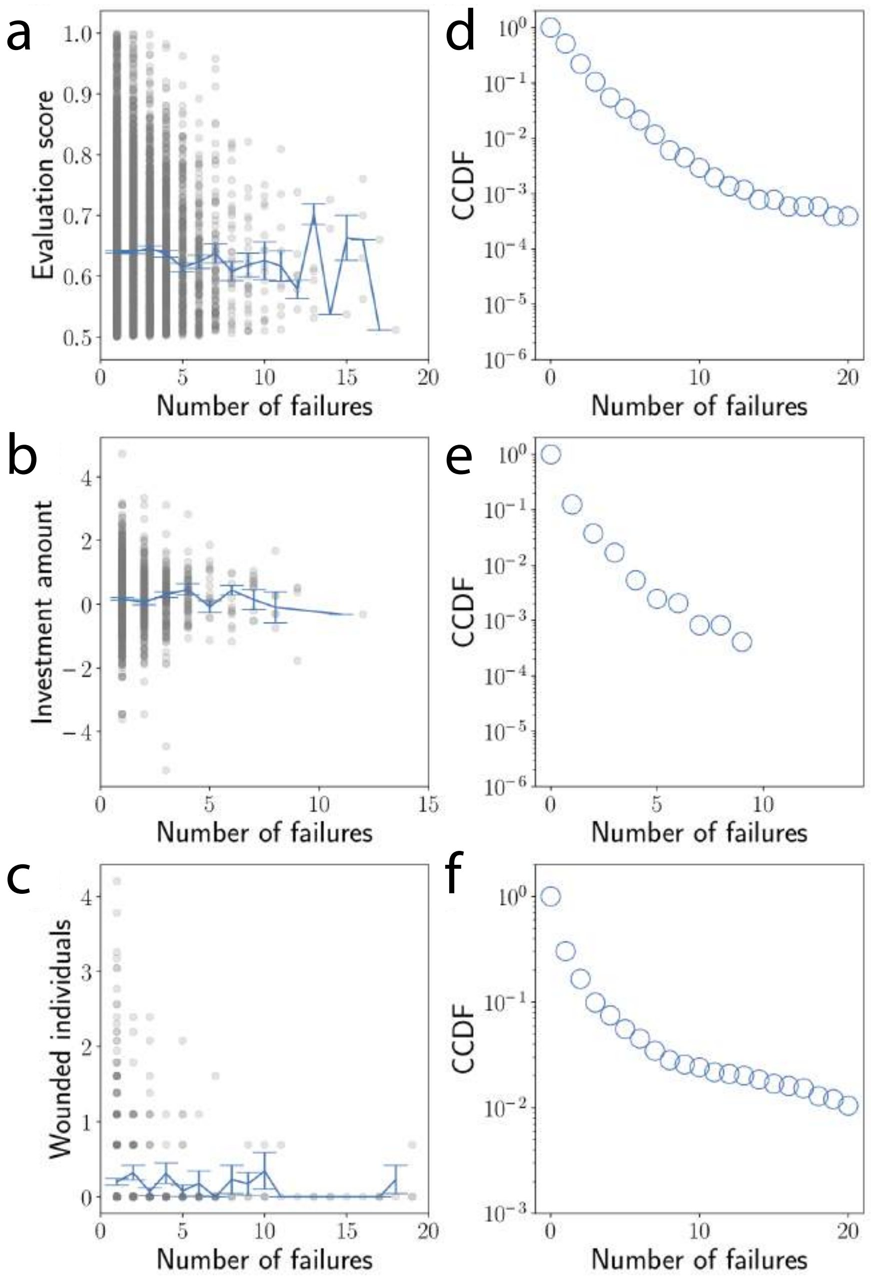


Figure S13: **Testing fitness hypothesis.** The correlation between length of failure streak and initial performance is weak (a-c, $r = -0.05, -0.01, -0.13$ respectively, not significant for $D_2$). We also find the length of failure streak still follows fat-tailed distributions conditional on bottom 25% initial performance samples (d-f, KS test between sample and exponential distribution rejects the two distributions to be identical with p-value $< 0.01$).

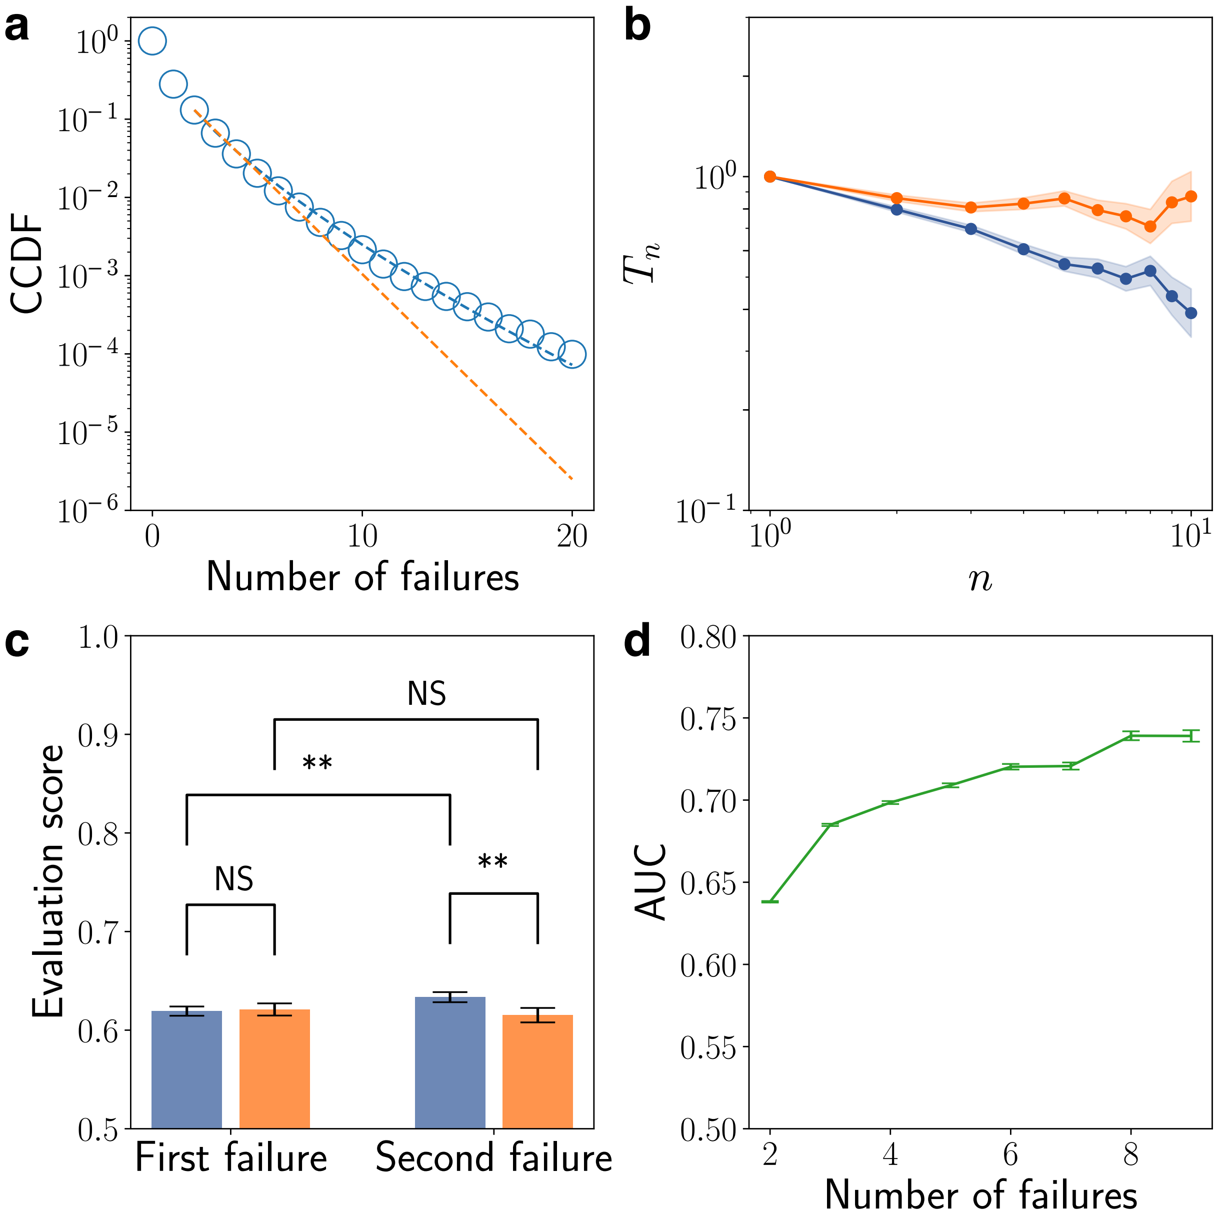


Figure S14: **Robustness checks on $D_1$ as we change the threshold of inactivity in the system to 2 years.** We repeat analysis on length distribution of failure streak (a), temporal patterns (b), performance divergence at the early stage (c) and predictability of eventual success (d), fining all these results still hold.

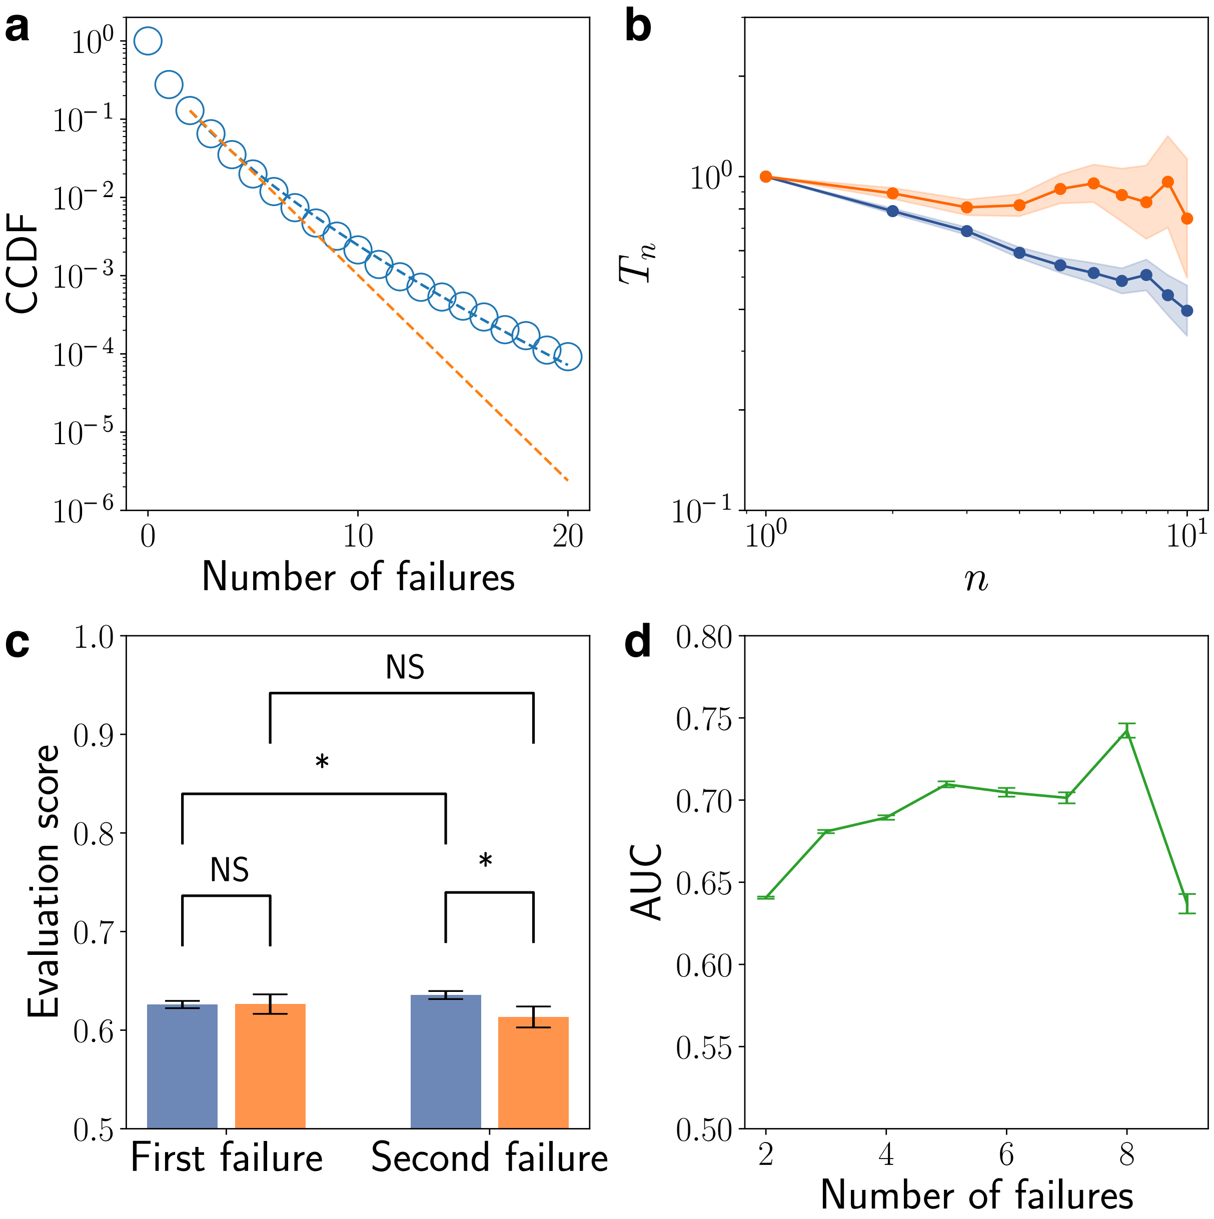


Figure S15: **Robustness checks on $D_1$ as we change the threshold of inactivity in the system to 8 years.** We repeat analysis on length distribution of failure streak (a), temporal patterns (b), performance divergence at the early stage (c) and predictability of eventual success (d), fining all these results still hold.

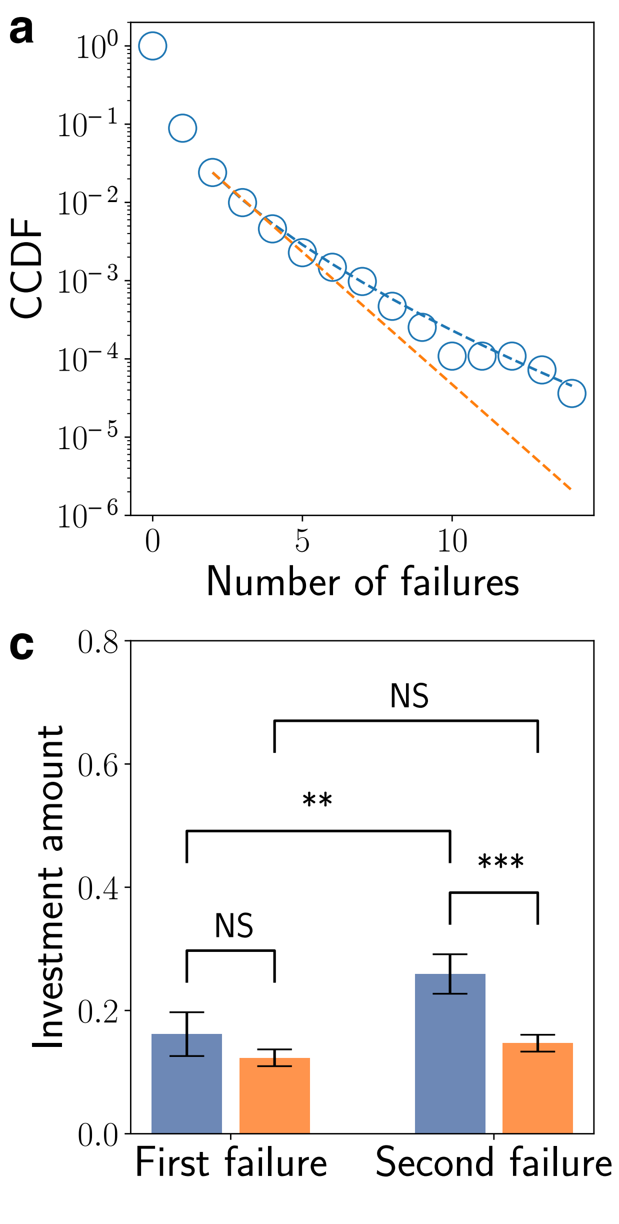


Figure S16: **Robustness checks on $D_2$ as we change the threshold of inactivity in the system to 2 years.** We repeat analysis on length distribution of failure streak (a), temporal patterns (b), performance divergence at the early stage (c) and predictability of eventual success (d), fining all these results still hold.

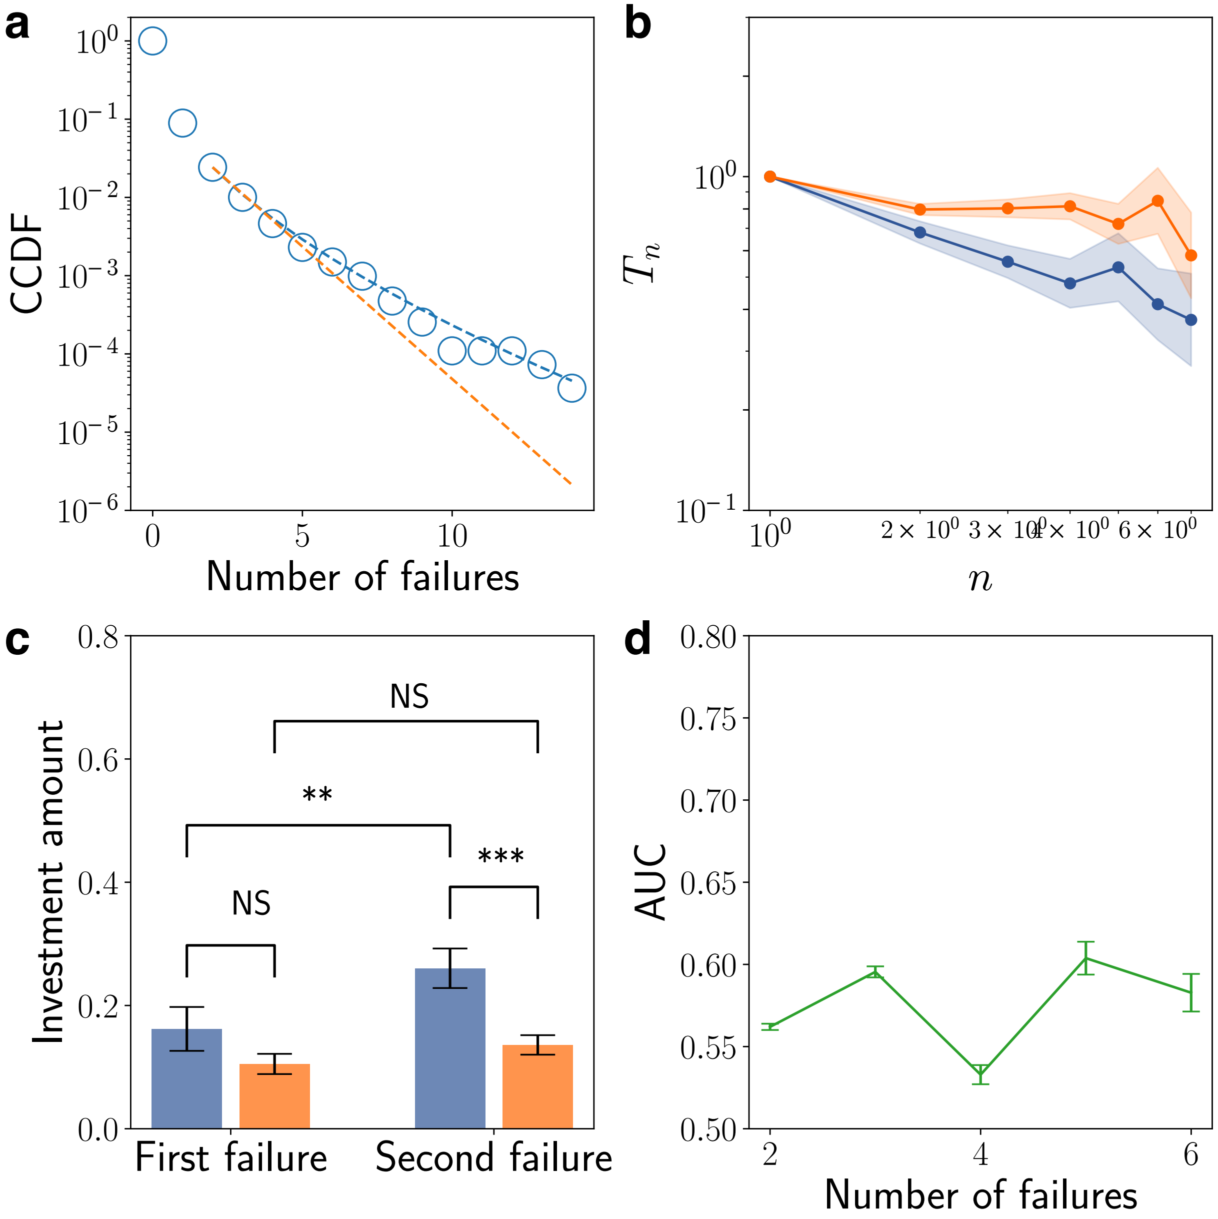


Figure S17: **Robustness checks on $D_2$ as we change the threshold of inactivity in the system to 8 years.** We repeat analysis on length distribution of failure streak (a), temporal patterns (b), performance divergence at the early stage (c) and predictability of eventual success (d), fining all these results still hold.

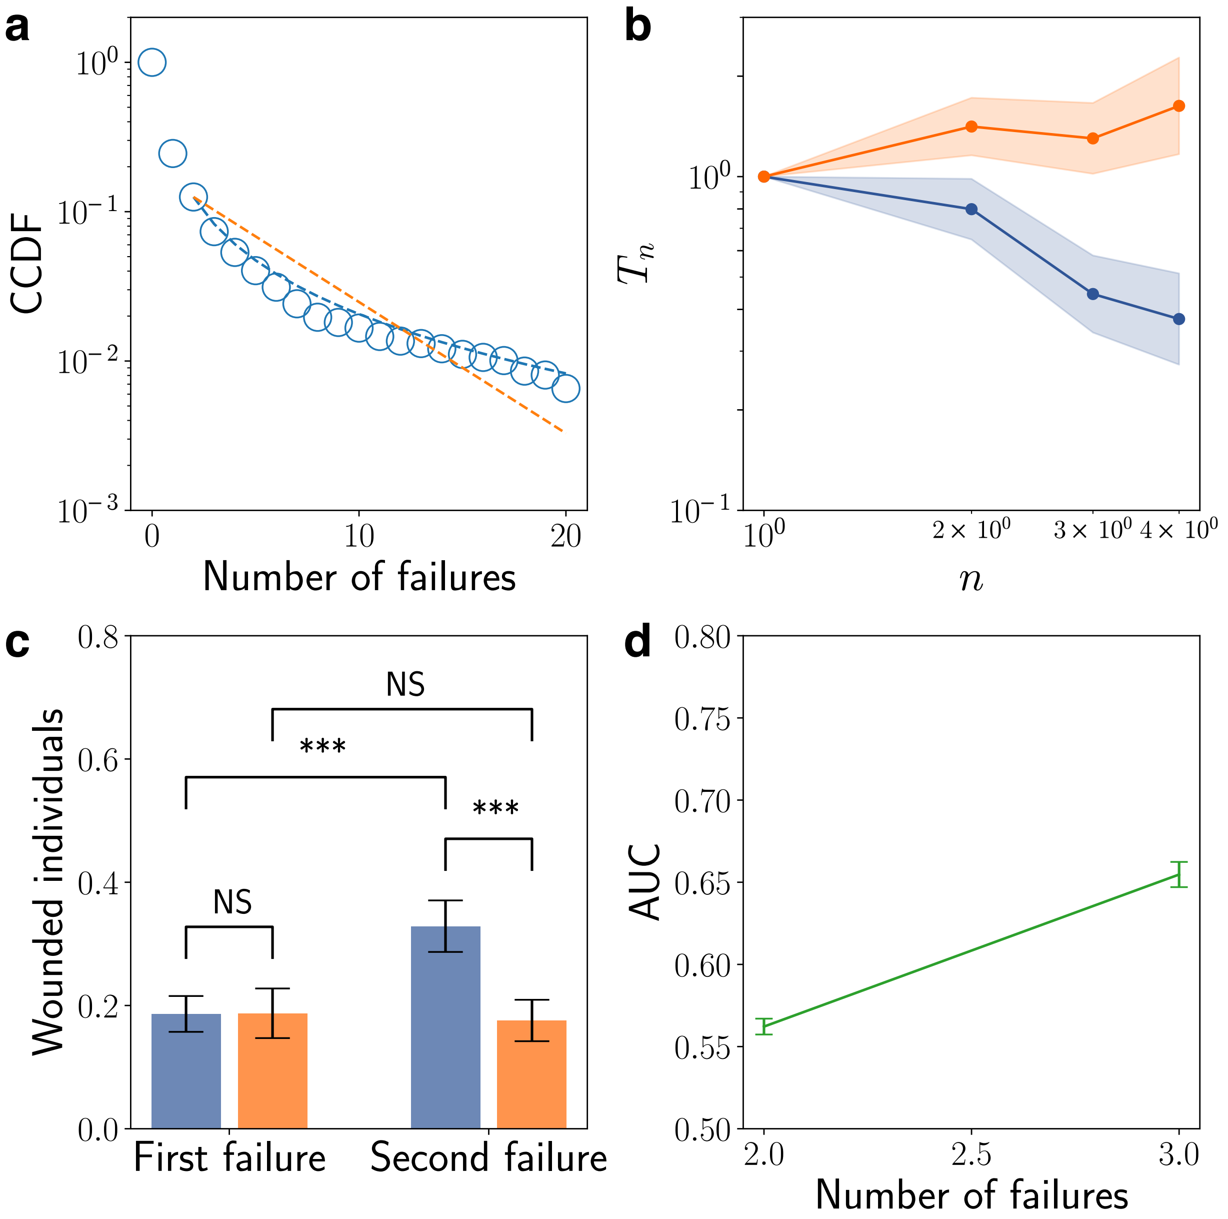


Figure S18: **Robustness checks on $D_3$ as we change the threshold of inactivity in the system to 2 years**. We repeat analysis on length distribution of failure streak (a), temporal patterns (b), performance divergence at the early stage (c) and predictability of eventual success (d), fining all these results still hold.

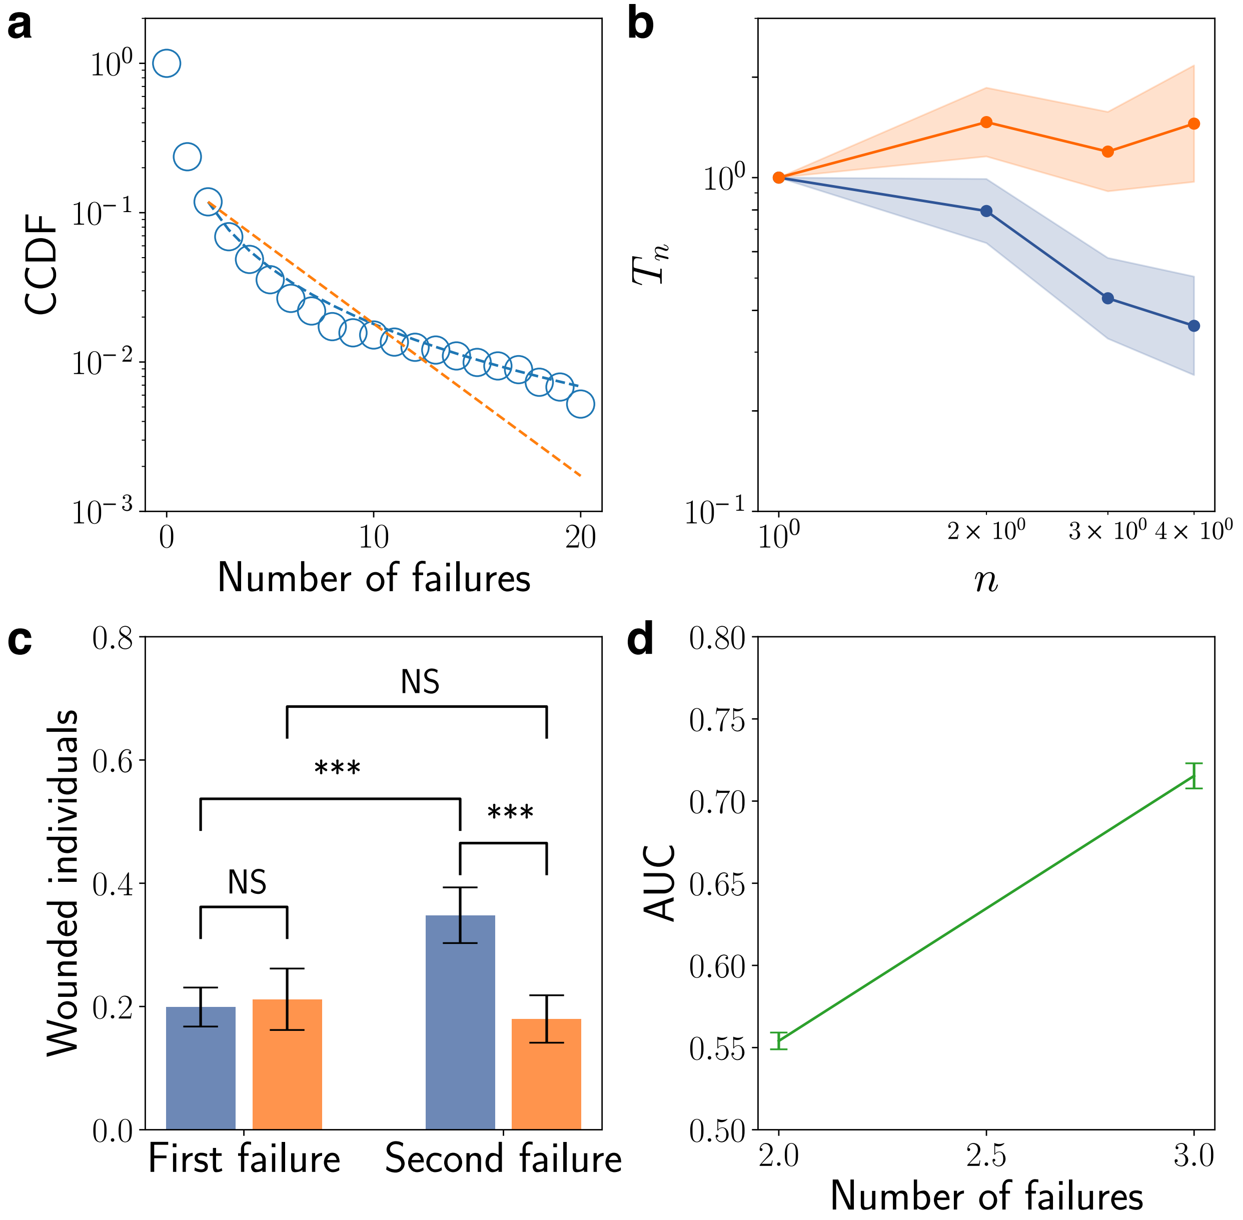


Figure S19: **Robustness checks on $D_3$ as we change the threshold of inactivity in the system to 8 years.** We repeat analysis on length distribution of failure streak (a), temporal patterns (b), performance divergence at the early stage (c) and predictability of eventual success (d), fining all these results still hold.

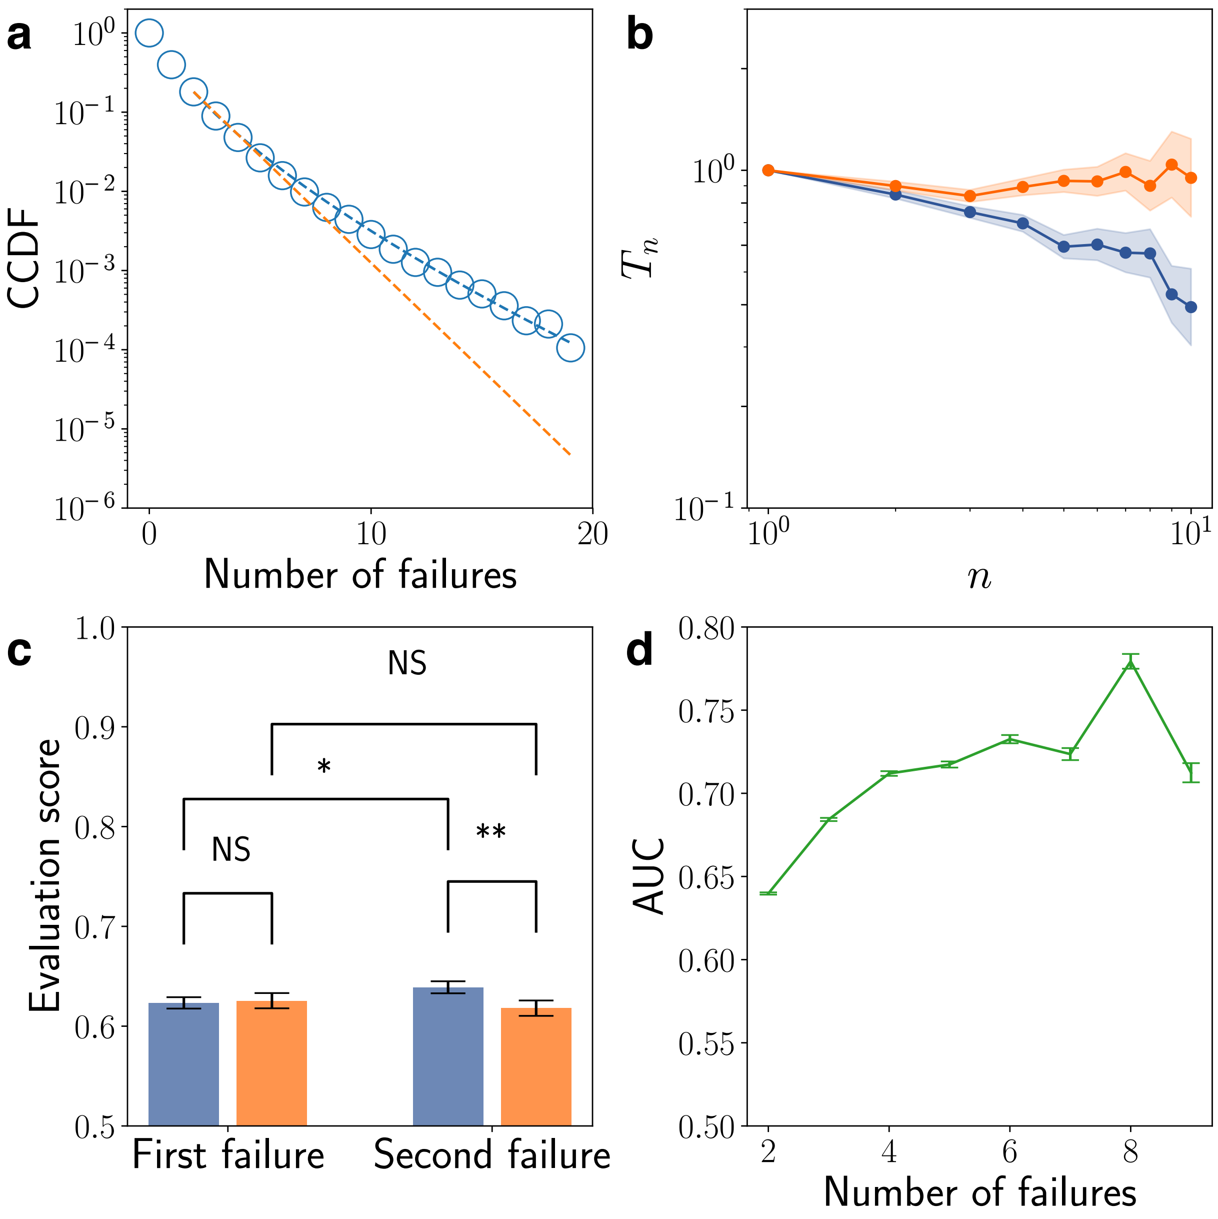


Figure S20: **Robustness checks on $D_1$ only excluding revisions as successes.** We repeat analysis on length distribution of failure streak (a), temporal patterns (b), performance divergence at the early stage (c) and predictability of eventual success (d), fining all these results still hold.

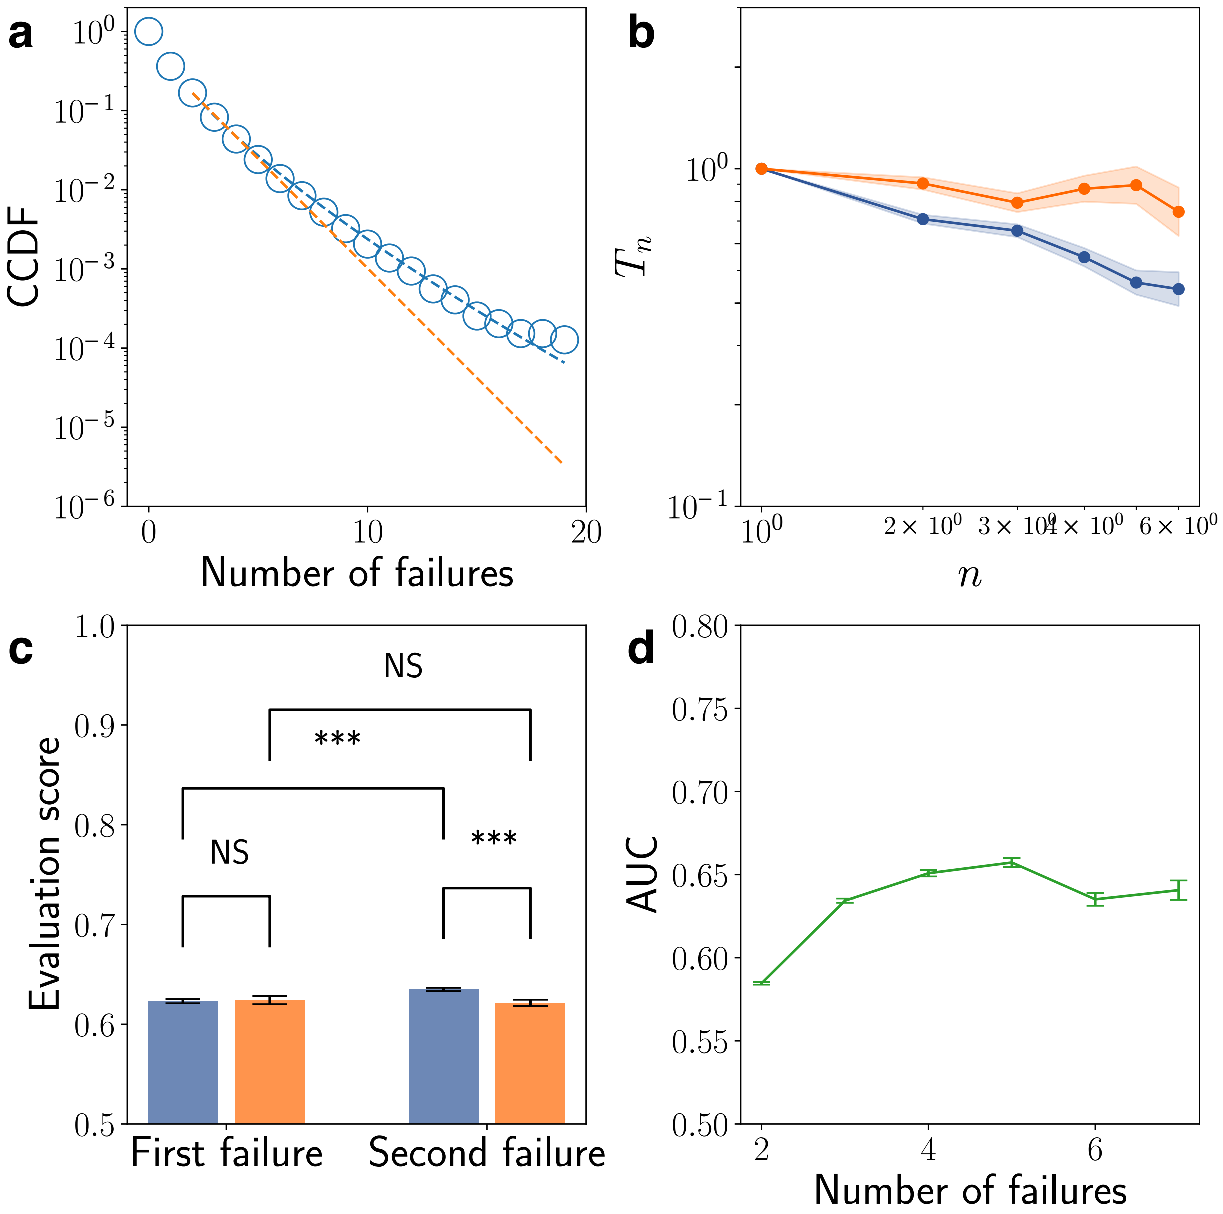


Figure S21: **Robustness checks on $D_1$ only focusing on samples before one's first R01 success.** We repeat analysis on length distribution of failure streak (a), temporal patterns (b), performance divergence at the early stage (c) and predictability of eventual success (d), fining all these results still hold.

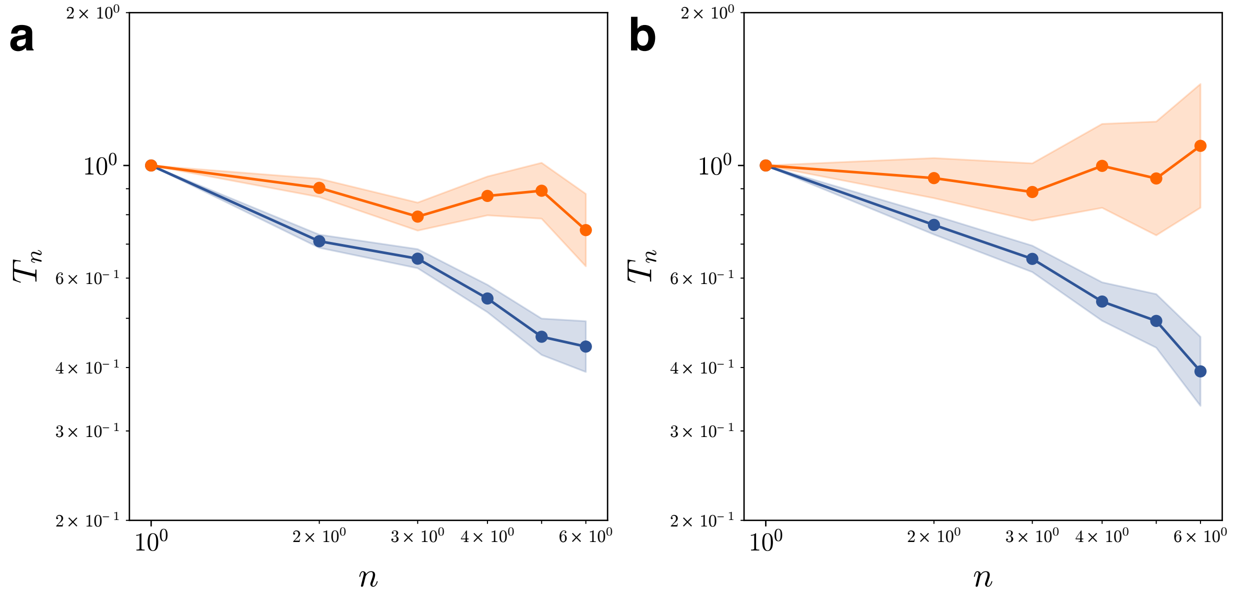


Figure S22: **Robustness checks on $D_1$ with respect to prior successes.** Here we measure samples with (a) and without (b) prior success, finding they show similar temporal patterns.

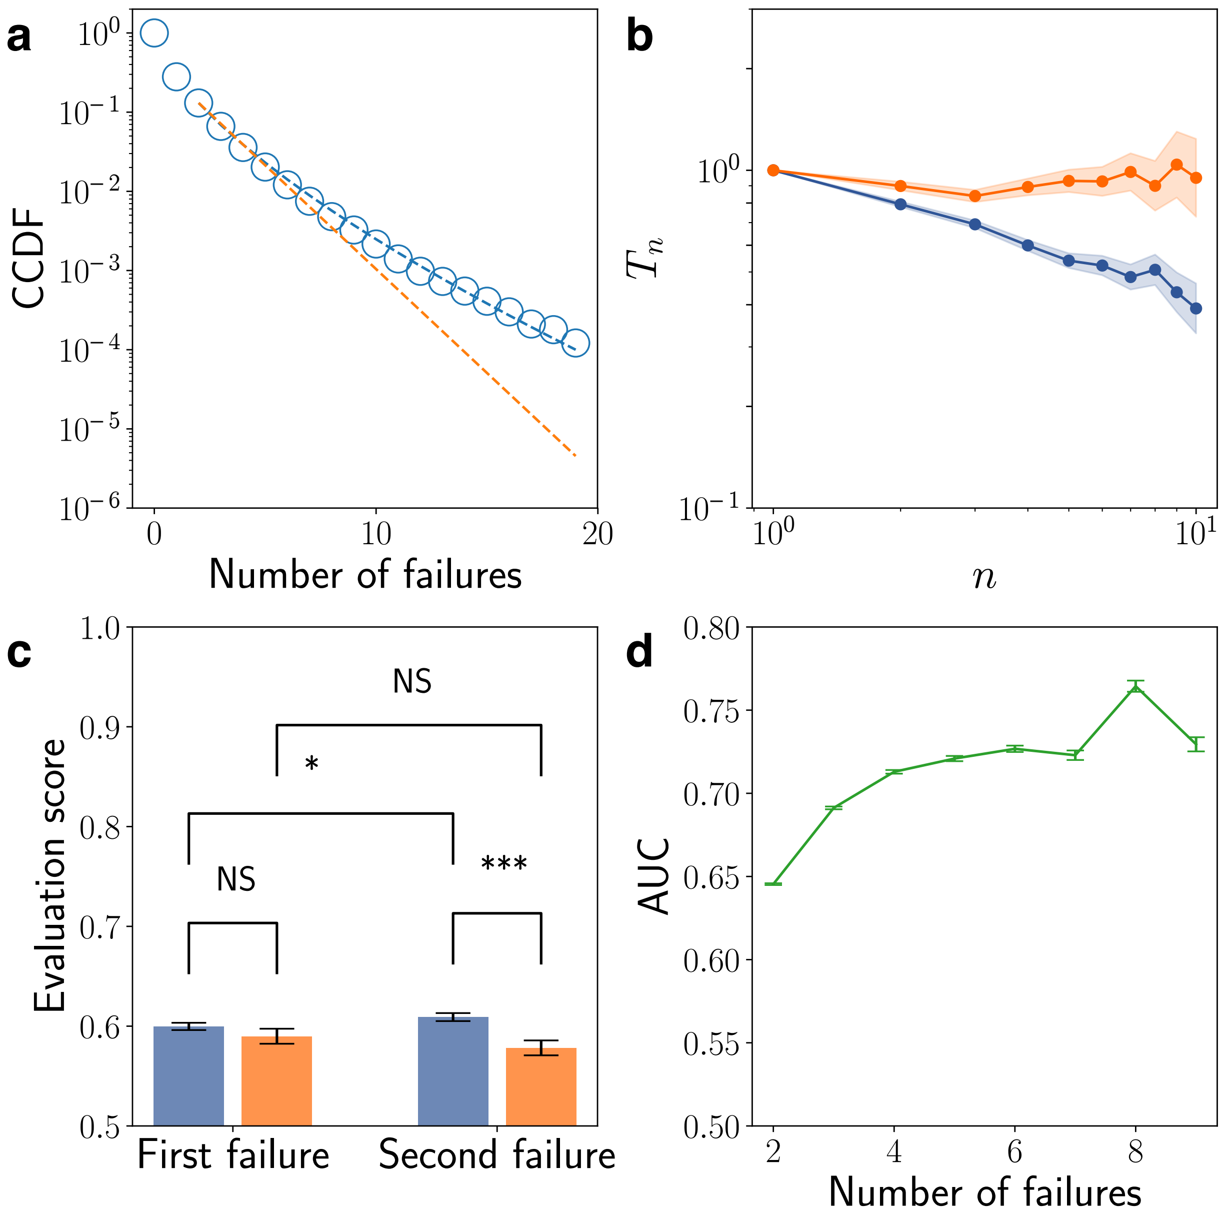


Figure S23: **Robustness checks on $D_1$ as we change the discuss score threshold to 55.** We repeat analysis on length distribution of failure streak (a), temporal patterns (b), performance divergence at the early stage (c) and predictability of eventual success (d), fining all these results still hold.

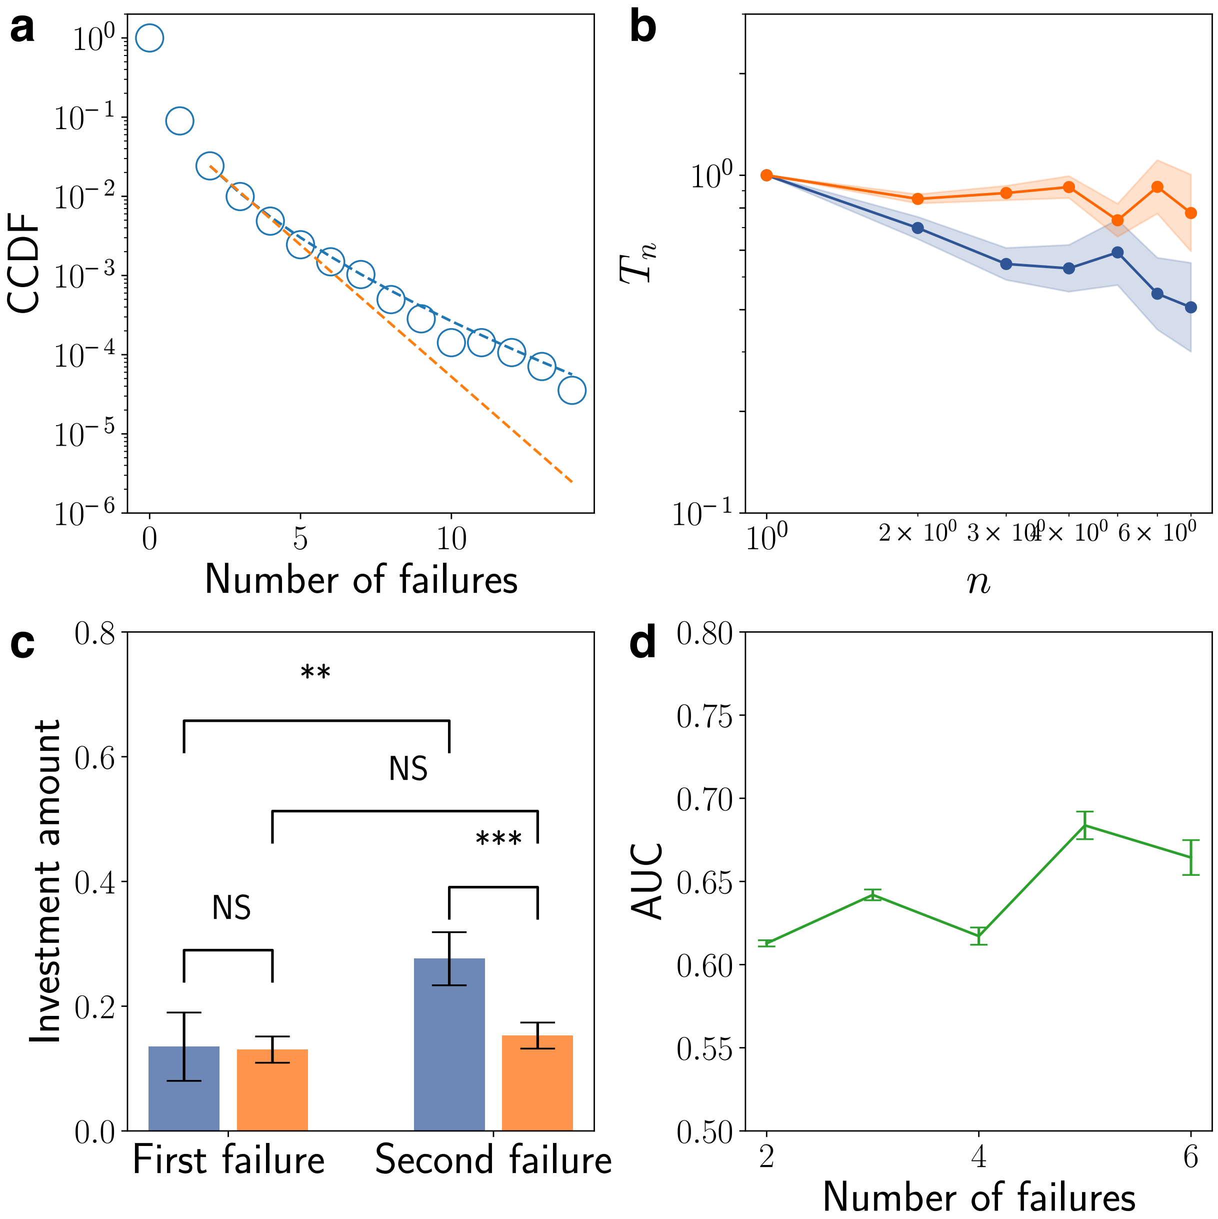


Figure S24: **Robustness checks on $D_2$ as we change the threshold of 'high-value M&As' as M&As that values ranking top 5% in the same year.** We repeat analysis on length distribution of failure streak (a), temporal patterns (b), performance divergence at the early stage (c) and predictability of eventual success (d), fining all these results still hold.

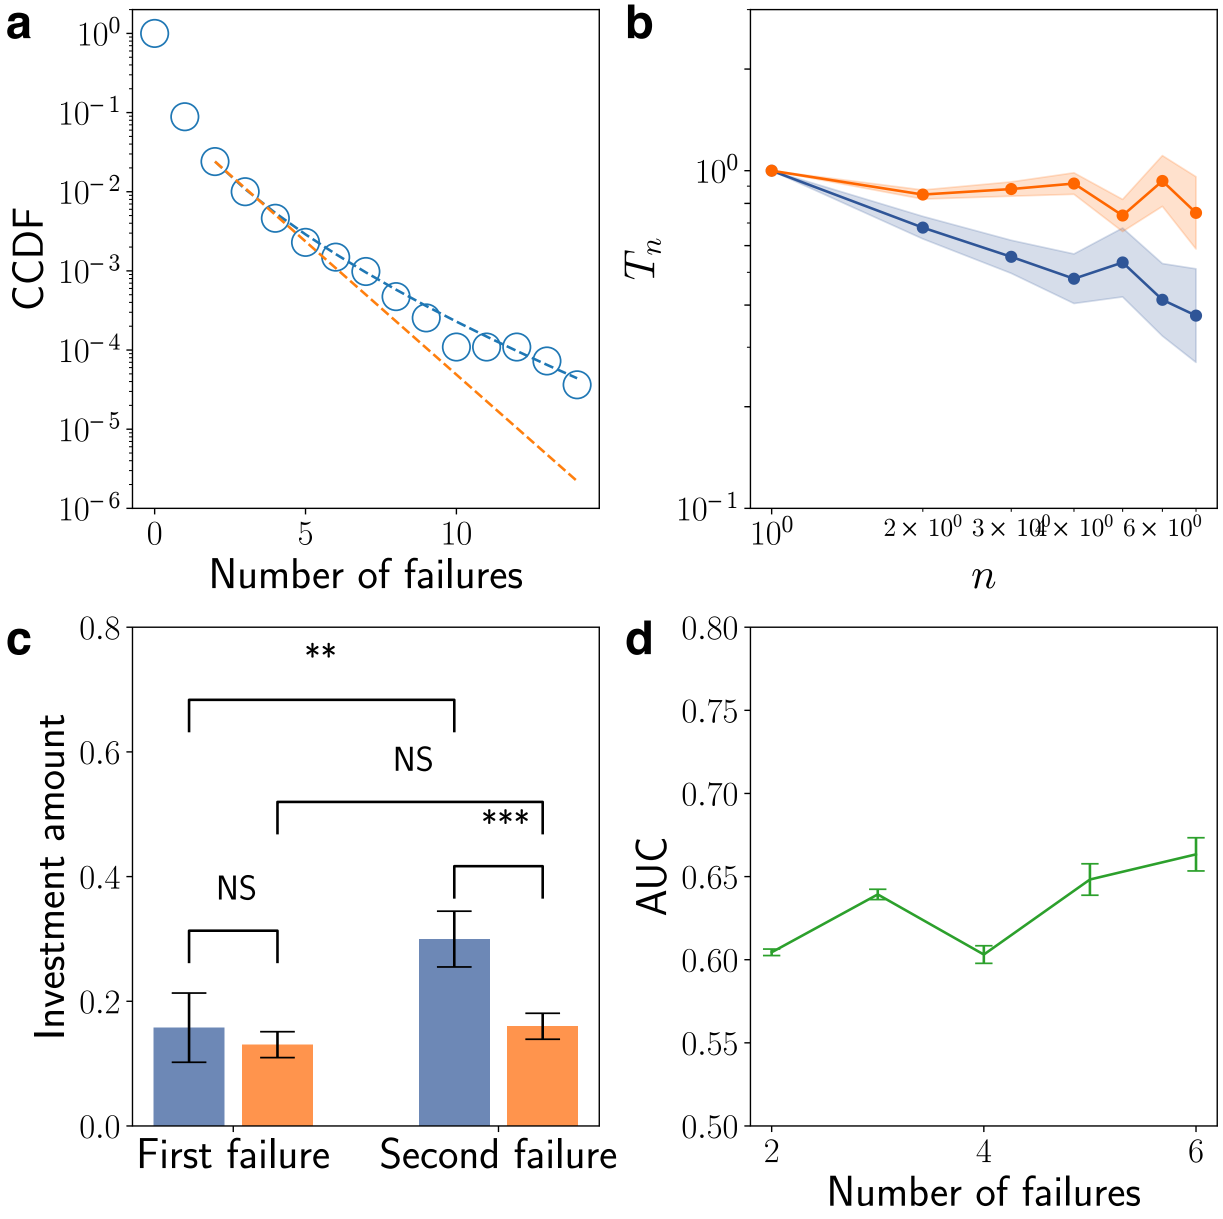


Figure S25: **Robustness checks on $D_2$ as we exclude all M&As and restrict success as companies that went public.** We repeat analysis on length distribution of failure streak (a), temporal patterns (b), performance divergence at the early stage (c) and predictability of eventual success (d), fining all these results still hold.

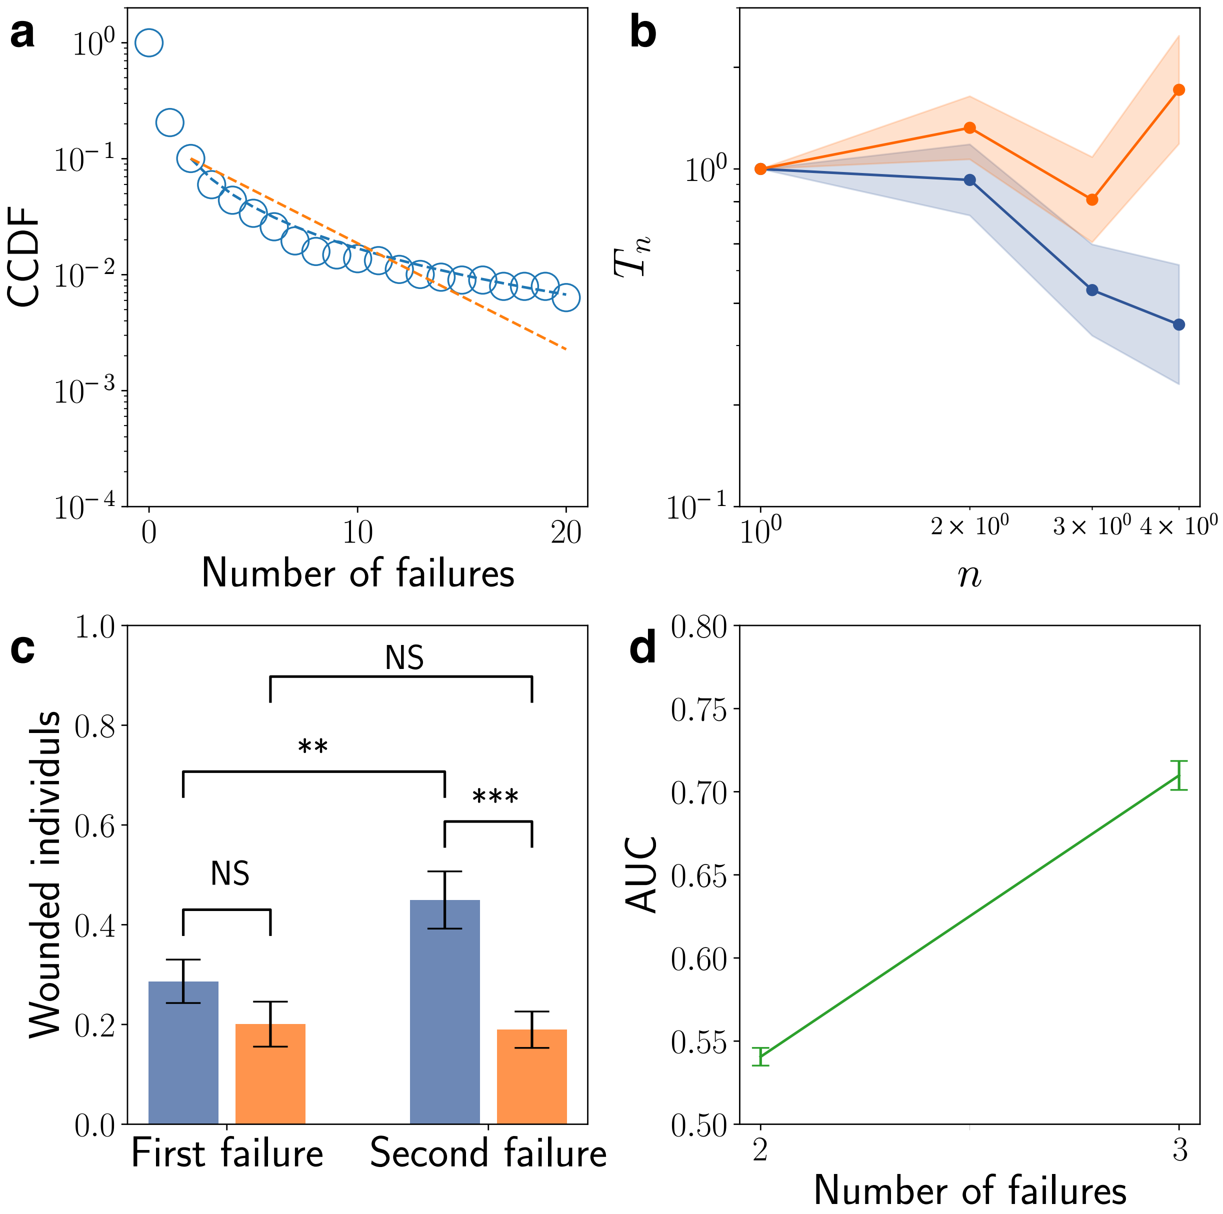


Figure S26: **Robustness checks on $D_3$ as we restrict the attack type to be aimed at human beings.** We repeat analysis on length distribution of failure streak (a), temporal patterns (b), performance divergence at the early stage (c) and predictability of eventual success (d), fining all these results still hold.

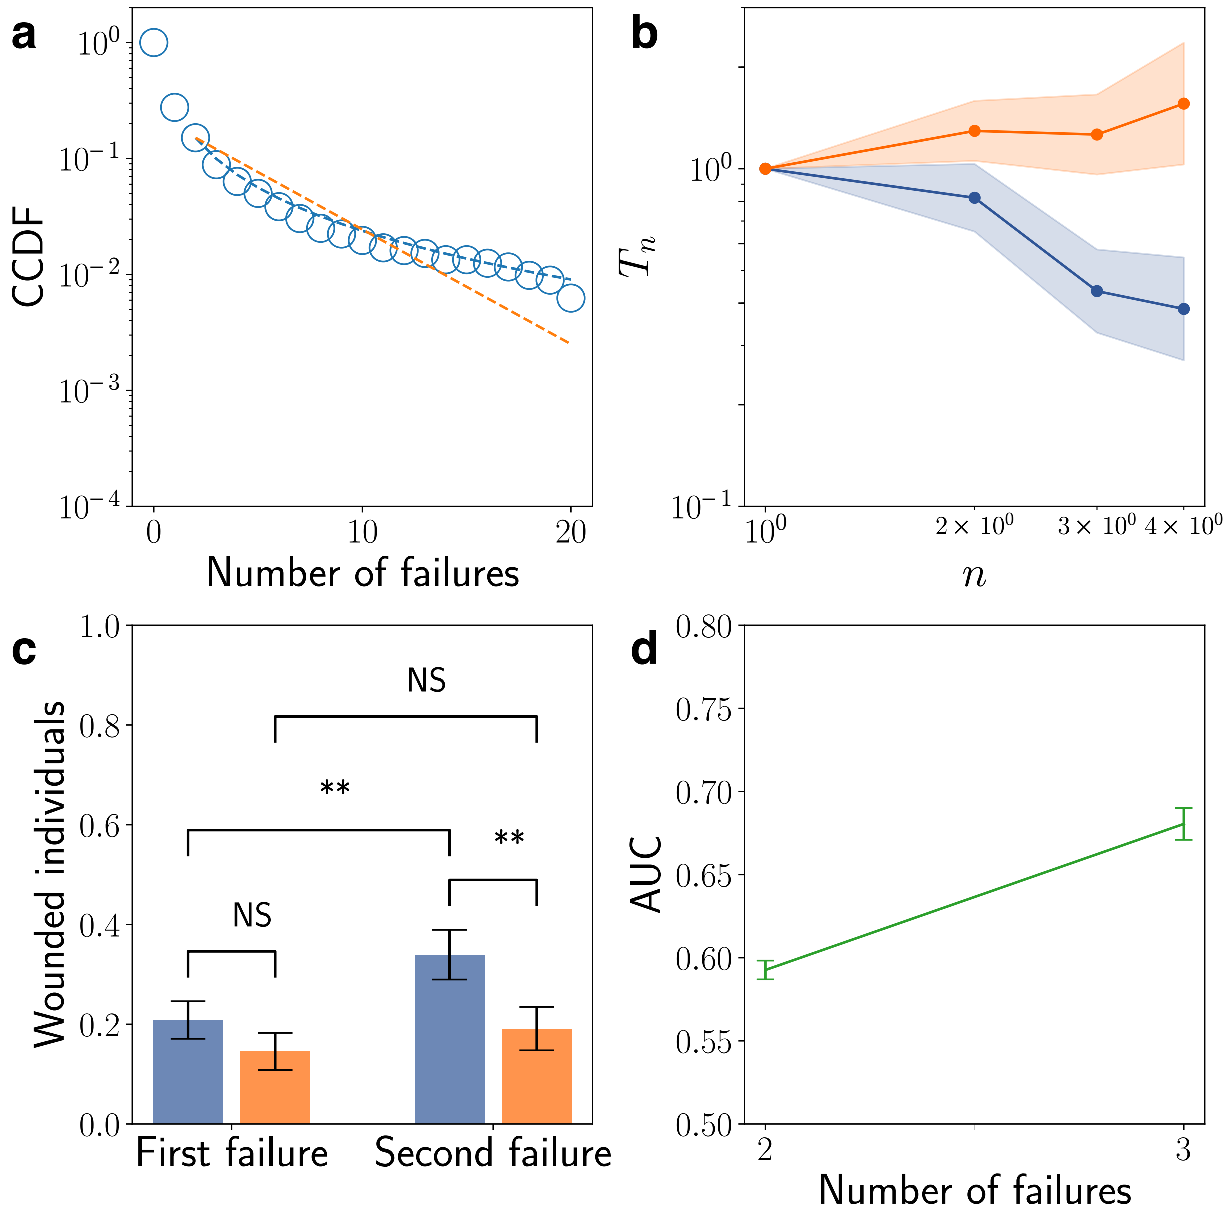


Figure S27: **Robustness checks on $D_3$ as we restrict our samples to be within in perpetrator group list.** We repeat analysis on length distribution of failure streak (a), temporal patterns (b), performance divergence at the early stage (c) and predictability of eventual success (d), fining all these results still hold.

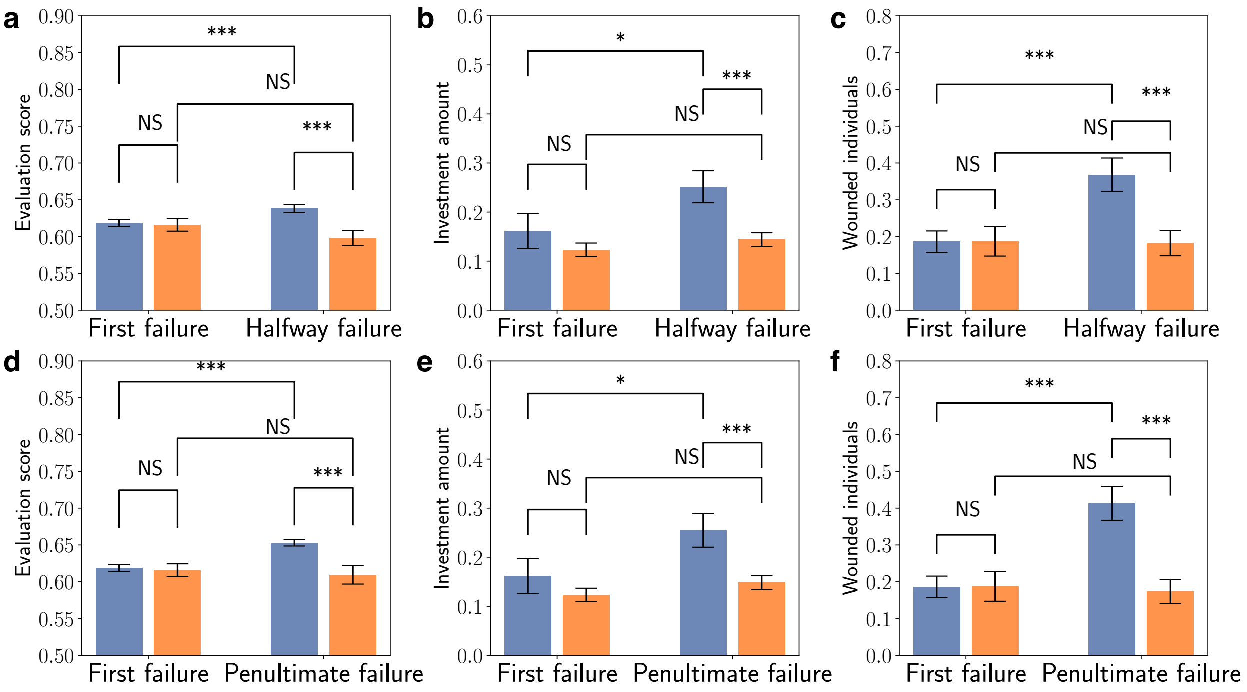


Figure S28: **Robustness checks for different failures.** Here we compare the performance dynamics between the first and halfway (a-c) and penultimate (d-f) failures across the three datasets, finding our results are broadly consistent with Fig. 4.
